# Supplementary material for: Dissolving the Fermi Paradox
Source: arXiv:1806.02404 ancillary file (2018-06-06)
Supplement: Supplementary file 1 [file supplement-i.pdf]

PROCEEDINGS A

rspa.royalsocietypublishing.org

Research

Article submitted to journal

# Supplement I: Biological transitions, alternatives, and uncertainties on paths to complex life

Anders Sandberg[1], Eric Drexler[1] and Toby Ord[1]

[1]Future of Humanity Institute

© The Authors. Published by the Royal Society under the terms of the Creative Commons Attribution License http://creativecommons.org/licenses/by/4.0/, which permits unrestricted use, provided the original author and source are credited.

THE ROYAL SOCIETY
PUBLISHING

## Introduction

As discussed in the main text, because of observer selection effects, our own existence *per se* places no quantifiable lower bounds on the prevalence of Earth-like planets, life, or intelligence. It is perhaps significant that currently popular models of cosmology propose that our universe is much larger than the volume we can observe and place no upper bound on its size.

Note that we are not arguing that life or intelligence is extremely rare, merely that, given our present state of knowledge of the origin of complex life, it could be common, rare, or extremely rare. As discussed in the main text, our conclusions rest not on low expected values of model parameters, but on large uncertainties (here given as estimated values of log uncertainty, LU) that extend to low values.[1]

Because model uncertainties are central to the present argument, is important to explore a range of competing hypotheses. To make a case for substantial uncertainty in origin-of-life models, the typical argument is not that "There is strong evidence for (or against) model $A$" but rather, that "It would be *unsurprising* if any one of the alternative models $A$, $B$, $C$ or $D$ were true", where this set of physically plausible alternatives collectively implies large LU. Likewise, regarding a distribution over potential values of a model parameter $X$, the typical argument is not that $X$ is *likely to be within* a given range, but that it would be *unsurprising* if $X$ were found to be *anywhere within* (or even substantially outside) a range that spans a large LU$[X]$.

We begin by reformulating origin-of-life models in physical terms, not attempting to directly estimate $f_l$ and $f_i$, but instead considering the general nature of processes that lead to transitions from abiotic to genetic systems, and from genetic systems to their potential successors. As discussed in the main paper, broad, weakly structured distributions over the physical process parameters imply highly non-uniform distributions over both $f_l$ and $f_i$.

## Reformulating origin-of-life models

On Earth, the path from the early abiotic environment to a world with advanced organisms passed through a series of transitions: first, an abiotic/genetic transition (AGT), followed by one or more genetic/genetic transitions (GGTs) of the kind discussed below. Any or all of these transitions could have been fast and highly probable on any of a wide range of planets, or slow and highly improbable on even the most favorable planets. What matters in the present context is that current uncertainties regarding the requisite chains of AGT and GGT processes introduce log-broad uncertainties in one or more of the model parameters, and that these uncertainties extend to parameter values that would imply that one or more critical AGT or GGT events occurs with low frequency.

Following Spiegel [1], we describe AGT events as physical transitions that occur at some rate per unit time per unit volume of a suitable prebiotic substrate. Opportunities for these events to occur are bounded by the time scales of planetary evolution.

Without loss of relevant generality, we can treat (respectively) substrate volumes and populations as averaged over time and weighted by an appropriate quality metric, and can treat transitions as discrete events, whether or not a particular transition process crosses a sharp, naturally-defined threshold. Again without loss of relevant generality, we can consider the AGTs to be events that produce organisms of kinds that transiently or permanently dominate subsequent planetary biospheres.

The probability of observing an AGT after time $t$ on a planet with a volume $V$ of substrate with an AGT rate of $\lambda$ transitions per unit volume and time is $p_l = 1 - e^{-\lambda V t} \approx \lambda V t$, where the approximation applies for small values. This represents an exponential decay of pre-transition

[1] One might worry that very low fractions of planets giving rise to life would violate the Copernican principle, making our location atypical. However, our location is already known to be extremely atypical. Less than one part in $10^{37}$ of the universe is near a planetary surface, yet this is where we find ourselves. This is simply due to a statistical selection effect: presumably beings like us could not have arisen anywhere else. Similarly, even if fewer than one in $10^{37}$ planetary surfaces give rise to life, we could only find ourselves on one that did.

states over time. The probability of observing life plus $n$ GGTs (occurring at rate $\mu$ per biosphere) after time $t$ is (assuming independence) $p_{L+} = (1-e^{-\lambda V t}) \int_0^t \lambda V e^{-\lambda V s} F(t-s;n,\mu) ds$, where $F(s;n,\mu) = 1 - e^{-\mu s} \sum_{k=0}^{n-1} (\mu s)^k/k!$ is the Erlang CDF. For small values this is $\approx \lambda \mu V t/n$.

The rate parameters in AGT and GGT stem from processes that contain multiplicative uncertainties, resulting in large LUs. Because AGT and GGT processes are qualitatively different, they will be considered separately.

## AGTs and the origin of genetic systems: $f_l$

The origin-of-life literature today contains diverse and conflicting hypotheses regarding the terrestrial AGT event, and current knowledge places few constraints on potential transition rates or on the nature of favorable environments. A recent publication [2] notes that "investigations on the origins of life are riddled with numerous controversial questions", including:

> "Did life originate only once, by accident, or is it the probable outcome of chemical evolution, which has frequently occurred elsewhere in the universe? Which property of living beings came first: their ability to reproduce and transmit information to progeny, their metabolic capacity, or their compartmentalization as individual entities?"

More generally, models of the origin of life (here identified with an AGT event) differ in the proposed nature of initial genetic systems and in the physical processes and required conditions for their emergence [2, 3, 4, 5, 6, 7].

### AGT time, volume, and volumetric-rate parameters

We will take Earth as a model for potential life-bearing planets, without explicitly examining the potential range of alternative planetary conditions; the effect of this range is implicitly subsumed into $n_e$.

### LU[t]

Our conclusions are insensitive to the estimated distribution of $t$ which we will take as a range $10^7 < t < 10^{10}$ years; the first interval is a relatively short scale for global geological change, while the second is a generous scale for the persistence of a stable planetary environment. This range suggests a reference $\mathrm{LU}[t] \approx 3$.

### LU[V]

A suitable substrate for abiogenesis must provide a set of conditions that together enable the abiogenic formation of biopolymers, but as noted by Luisi [8], key constraints on this process (and hence the requisite conditions) are often ignored in the literature. For example, some models postulate the formation of peptide [9] or nucleic acid [10] polymers in aqueous solutions, then ask how a peptides might give rise to catalytic cycles of peptide synthesis, or how potential genetic material like RNA might template self-replication in aqueous solutions of monomers [4, 11, 12]. In their naÃŕve form, such models encounter a fundamental difficulty, because the formation of biopolymers from their monomers is forbidden in water solution [13]: Thermodynamic driving forces favor the reverse process, depolymerization by hydrolysis [2]. Extant biological systems overcome this difficult by synthesizing polymers, not from simple monomers, but from activated, thermodynamically-unstable precursors produced by energy-driven metabolic pathways.

A potential alternative, abiotic mechanism for polymerization is physical: Amino acids polymerize when dried and heated, hence cycles of drying and wetting could potentially deliver organic polymers to an aqueous solution in an abiotic environment [13]. Models that call for drying and heating suggest that abiogenesis may be constrained to repeatedly wetted films

at the margin of bodies of water, perhaps with a further requirement for geothermal heating. Considering representative values, the gap between these models (e.g., $10^7\,\mathrm{m}^2 \times 10\,\mu\mathrm{m}$ depth = $10^5$ l) and those that propose deeper substrates distributed over a large fraction of a planetary surface (e.g., $10^{14}\,\mathrm{m}^2 \times 1\,\mathrm{cm}$ depth = $10^{15}$ l) suggests a reference $\mathrm{LU}[V] \approx 10$.

The formation of polymers also requires substantial concentrations of monomers, and as Luisi notes, "The concentration threshold for prebiotic reactions is often not taken into account in the literature." [8] This is a strong constraint that greatly increases $\mathrm{LU}[V]$.

Carbonaceous chondrite meteorites (the best-studied abiotic reservoirs of relevant monomers) typically contain mixtures of >50 significant components, most at concentrations <10 ppm [14], while chemists undertaking the synthesis of biopolymers typically work with combinations of a few pure compounds at concentrations that are orders of magnitude higher. On entropic grounds, it would be surprising to find that a substrate with such dilute mixtures of compounds could support AGT events at substantial rates: bimolecular reaction rates, for example, scale as the square of reactant concentrations, hence reducing concentrations by $10^3$ reduces the rate of molecular encounters per unit volume by $10^6$, with a corresponding adverse shift in equilibrium product concentrations and downstream reaction rates.

Geochemical processes can, however, greatly concentrate chemical substances; for example bismuth is present at a mean concentration $C < 1$ ppm of Earth's crust [15], yet occurs as a native mineral in nearly pure form; elements such as silver, gold, and platinum likewise occur in nearly pure form, despite mean concentrations $C < 100$ ppb. Low mean concentrations of a substance, however, ensure that high concentrations are rare, and conjunctions of high concentrations of different substances can be yet more rare.

In an illustrative model, if conditions for abiogenesis were to require that geochemical processes concentrate a component of an initial mixture by a factor $R$, then the fraction of the initial volume that contains the resulting concentration will be $F < 1/R$, and typically much lower. If we model concentration ratios as uncorrelated, the fraction of potential substrate $F$ that contains $N$ required components (amino acids, nucleobases, ribose, phosphate?) at a concentration ratio $R$ would be $F < (1/R)^N$; $N = 20$ and $R = 1000$, would yield $F_{all} < 10^{-60}$. Because both concentration requirements and concentration processes are undetermined, the downward constraints on $\log(F_{all})$ are extremely weak.

The current state of knowledge of AGT processes (which includes extensive model uncertainties[2]) by no means excludes the possibility that chemical pathways might cross the abiotic/genetic threshold with less stringent conditions for geochemical separation and concentration, thereby permitting relatively large values for $V$. In light of these considerations, it seems difficult to argue for a value of $\mathrm{LU}[V]$ less than 50.

## LU for the AGT volumetric rate parameter

The greatest contributor to uncertainty regarding planetary AGT rates is the volumetric rate parameter $\lambda$, because the emergence of viable genetic systems might be incremental and deterministic, or might require a combination of rare events.

A parallel can be drawn between AGTs and protein folding, in that both AGT events and protein folding events require the emergence of an ordered state from disordered monomers. In the case of protein folding, monomers form a chain with a sequence selected from an immense

[2]For example, there has been little or no exploration of models in which information transmission in primitive genetic systems is mediated not by DNA-like polymer-polymer complementarity, but by molecular imprinting in organic or inorganic materials (a role for imprinting mechanisms in the emergence of metabolism was suggested in [16], but received no notable follow-up). Imprinting has several intriguing features: The binding specificity of molecular imprints has been compared to that of antibodies [17, 18], and like antibodies, imprints can mediate chiral separations [19] and perform catalysis [17]. Imprinting in films on mineral surfaces would be compatible with amino acid polymerization driven by cycles of wetting and dehydration [13], and cycling conditions could provide a mechanism for molecular binding and release, potentially enabling imprint-templated polymers to form next-generation imprints. By avoiding the need for a small repertoire of complex, complementary, chiral monomers, imprint-based models could potentially resolve the genes-first vs. metabolism first puzzle noted above, while the potential replication of surface-anchored dendrimeric structures suggests a membrane-free mechanism for combining diverse molecular functionalities in a (pre-)biological unit.

combinatorial space by an incremental evolutionary process, yet that sequence does not directly determine the folded structure. Because the conformation of peptide bond between a pair of amino acid monomers is characterized by both $\phi$ and $\psi$ bond angles, each of which may take on any of 3 stable conformations, folding (e.g., of a 300 residue sequence) can be seen as a Brownian search through a space of $> 10^{285}$ conformational states. If a random sequential search were to sample, for example, $10^{12}$ conformational states per molecule per second, the waiting time for a folding event in an oceanic volume of a high-concentration protein solution would be $>10^{249}$ s ($\gg 10^{200}$ times the present age of the universe). In reality, however, individual protein molecules typically fold within seconds. This enormous disparity [20] has been termed "Levinthal's Paradox" [21].

Protein folding avoids Levinthal's Paradox because conformational dynamics is biased by a free-energy distribution that declines along many paths that lead to the folded state, a so-called "funnel" in the energy landscape [22]. Protein folding is a funnel-directed process in this sense because partial folds are more stable than random conformations, and can serve as intermediates on paths to the fully-folded state.

At present, there is no concrete evidence or widely-accepted principle that indicates whether AGT events entail processes that are random and Levinthal-like, or convergent and funnel-like. By definition, however, a pre-AGT world lacks a genetic evolutionary process, hence the mechanism that has ensured fast protein folding cannot operate. Nonetheless, we cannot exclude the possibility of alternative mechanisms, not genetic in a conventional sense, that would accumulate substructures through convergent, funnel-like processes [12, 16, 23].

An additional, powerful consideration is a difference in the number of target end-states: While the target for a protein folding event is a unique functional structure, the target for an AGT event could be any member of a space of potential initial genetic structures that, like the space of functional protein *sequences*, is itself of combinatorial scale.

Inasmuch as a molecular system at the AGT threshold is likely to be far more complex than a single protein, and proposed funnel-like processes are speculative, taking $\mathrm{LU}[\lambda] > 300$ as a reference value seems conservative. To claim confidence that $LU$ is less than 300 would be bold, even allowing for a combinatorially large set of alternative AGT paths and outcomes.

An *extremely* conservative upper bound on $\lambda$ is the frequency of bacterial cell division per bacterial volume, $\approx 10^{-3}\,\mathrm{s}^{-1}\,\mu\mathrm{m}^{-3} = 10^{12}\,\mathrm{l}^{-1}\,\mathrm{s}^{-1}$. Taking this value as the upper bound of a range with $\mathrm{LU}[\lambda] > 200$ would place the lower bound at $< 1 \times 10^{-188}\,\mathrm{l}^{-1}\,\mathrm{s}^{-1}$, and folding in high-end values for $V$ ($10^{15}$ l) and $t_{orig}$ ($10^{17}$ second) would yield a value of $f_l \approx \lambda V t_{orig} < 10^{-156}$. Using the same high-end value of $V t_{orig}$ , any value of $\lambda$ substantially greater than $10^{-32}\,\mathrm{l}^{-1}\,\mathrm{s}^{-1}$ would yield $f_l \approx 1$.

It is useful to note that log-broad distributions over $f_l \approx \lambda V t_{orig}$ imply log-broad distributions over the ratio of outcomes, $\Pr(\mathrm{AGT})/\Pr(\mathrm{noAGT})$, which can be thought of as a branching ratio (given as a log-ratio, $\mathrm{LR}^{a/b}[G] = \log(G_a/G_b)$) between biotic and abiotic worlds. For uniformity of notation, we denote the branching ratio for a transition to an initial genetic system on a potential path to complex life as $\mathrm{LR}^{+/-}[G_0]$. For reference calculations, we will take $\mathrm{LU}[\lambda V t_{orig}] > 200$, and note that $\mathrm{LR}^{+/-}[G_0]$ extends to low values (e.g., $\mathrm{LR} < 100$).

## GGTs and alternative genetic systems: $f_i$

In the terrestrial history, the evolution of complex life traverse a path that led from a direct products of an abiotic-genetic transition through a series of one or more through one or more genetic-genetic transitions (GGTs). Uncertainties regarding the rates and results of GGTs play a large role in the $LU$ for the parameter $f_l$.

Without loss of relevant generality, we can treat genetic-genetic transitions (GGTs) as events that produce organisms of kinds that transiently or permanently dominate subsequent planetary biospheres, and can treat GGTs as discrete events, whether or not a particular transition process crosses a sharp, naturally-defined threshold. One could follow the AGT model and describe GGT events as transitions that occur at some rate per unit time per unit population of organisms

evolving within some time interval. However, because GGT uncertainties are better described in terms of branching ratios between competing transitions, it is more natural to frame the discussion in terms of the alternatives (e.g, $A$ and $B$) and

distributions over outcome ratios, with values of log-ratio, $LR[A/B]$, and log-uncertainty, $\mathrm{LU}[A/B]$, in the value of LR.

In terrestrial biology, the organization of molecular machinery in current organisms strongly suggests that the machinery of ribosomal translation systems (through which nucleic acids encode and direct the synthesis of proteins) emerged through a GGT from biological systems in which nucleic acids served as both genetic and functional materials. According to the widely accepted "RNA-world" hypothesis [4, 12], RNA-based "ribozymes" played roles like those of today's ribosomally constructed, protein-based enzymes. A key piece of evidence for an early RNA world is that the core mechanism of the ribosome itself consists of strongly-conserved RNA structures; the recent demonstration of the amplification of RNA sequences by an RNA-polymerase ribozyme [24] reinforces evidence for the feasibility of an RNA-based biochemistry that lacks translational protein synthesis.

Because the history of terrestrial life includes at least one major GGT, it is important to consider the implications of potential alternative genetic systems and GGTs for the emergence of complex life and intelligence. The properties of GGTs indicate that rate parameters in this process should be assigned large values of LU.

## Evolutionary potential and $f_i$

In terrestrial history, complex life evolved from the last universal common ancestor (LUCA, a prokaryote in the post RNA-world) through a series of stages; notable milestones include the emergence of cells with mitochondria and nuclei (eukaryotes) and of multicellular animals (metazoa). The geological record shows that a span of some $\approx$4 Gyr of evolution stands between LUCA and us, with transitions from from LUCA to eukaryotes to metazoa to hominids at intervals of (respectively) $\approx$2 Gyr, $\approx$1 Gyr and $\approx$1 Gyr, preceded by a interval between Earth's origin and LUCA estimated as $\approx$0.5 Gyr.

Molecular and cellular processes (e.g., replication) typically operate on time scales of seconds or days, and knowledge of those processes would in itself provide no firm basis for predicting evolutionary delays on a time scale of $\approx$1 Gyr rather than 0.01 or 100 Gyr; knowledge of terrestrial biology provides even less basis for estimating the potential rate and scope of evolution in biologies based on alternative genetic systems.

We will use the term "evolutionary capacity" to refer to differences in rate and scope that would enable or preclude the evolution of complex life on a time scale $\leq$10 Gyr. Low evolutionary capacity might result either from slow evolutionary change, or from a ceiling on potential biological complexity.

It is plausible that the absence of systematic, ribosomal translation of genes to proteins would place a low ceiling on accessible biological complexity. It is likewise plausible that alternative genetic chemistries would increase or decrease the accessibility of translational systems, and that, among alternative translational systems, fundamentally different genetic codes might differ substantially in evolutionary capacity (e.g., through differences in coding capacity, or in accessible paths through genetic sequence space).

The prevalence of genetic systems with substantially higher or lower evolutionary capacity than terrestrial life would increase or decrease $f_i$. In particular, systems with a substantially restricted evolutionary scope would preclude intelligence, while systems with an evolutionary rate reduced by a log-factor of 4 would delay the emergence of intelligence to a time beyond the age of even the oldest stars.

## GGTs and alternative genetic systems

It has long been known that the range of potential alternative genetic systems extends beyond trivial differences in the assignment of codons to amino acids, and Crick has observed that that

**Table 1.** Alternative backbone and nucleobase chemistries

| Classes of alternatives | Accessibility considerations | Downstream implications |
|---|---|---|
| Glycol in place of sugar | Simpler metabolism, greater duplex stability | Variable, unknown |
| Different sugars | Variable (metabolic simplicity? duplex stability?) | Variable; potentially enable facile transcript modification |
| Amide linkages | Metabolism shared with peptides | Variable; alternative charged groups (amine, carboxylic acid) would enable facile transcript modification |
| Different nucleobases | Variable, unknown | Richer transcript chemistries, expanded codes? |
| Ionic pairs | Metabolic simplicity, stronger binding | Amine/carboxylic acid transcript chemistries, facilitation of non-translational genetic systems? |

"the adaptor hypothesis [synthesis mediated by tRNAs] allows one to construct, in theory, codes of bewildering variety" [25] Laboratory experiments suggest further potential differences not only in the organization of coding systems, but in the presence or absence of translation-mediated encoding, and in the chemical nature of the genetic material itself.

We will group salient alternatives into three classes:

*Alternative backbone and nucleobase chemistries:* Terrestrial genetic molecules employ backbones based on phosphodiester-linked deoxyribose and ribose sugars together with 5 nucleobases (of which DNA and RNA each use 4); alternative chemistries have been demonstrated in laboratory experiments.

*Alternative encoding systems:* The codons corresponding to amino acids are contiguous (neither overlapping nor separated by "commas"), and consist of words of length 3 written in a 4-letter alphabet; alternative encodings have been demonstrated in laboratory experiments.

*Alternatives to translated genetic codes:* The modern genetic system uses ribosomal machinery, tRNA molecules, and aminoacyl tRNA synthetase enzymes to translate sequences of codons into sequences of amino acids; neither the peptide sequence nor its structure has a direct, chemical connection to the genetic molecules. Chemical principles and laboratory experiments suggest alternatives.

We find multiple alternatives in each class, and any of these (or other alternatives) could potentially both dominate GGT pathways and yield systems that differ critically in subsequent evolutionary capacity.

## Alternative backbone and nucleobase chemistries

There is good reason to think that DNA/RNA genetic systems were preceded by a series of one or more genetic systems that employed nucleic acids with simpler backbone structures [26] [2], e.g., based on an achiral, 3-carbon molecule, propylene glycol [27, 28], rather than on a chiral, 5-carbon ribose or deoxyribose sugar (a problematic requirement [29]). Experiments have demonstrated a wide range of potential alternative backbone structures that support Watson-Crick base pairing [30, 31, 32]. Backbone structures that support self-complementarity, but not complementarity to terrestrial nucleic acids, would constitute broad range of alternative genetic chemistries that would have difficulty accessing GGTs that could lead to the terrestrial system.

A more radical alternative would avoid sugar-phosphate backbones in favor of amide-linked monomers like those of peptides. Such polymers (so-called "peptide nucleic acids" [33])

**Table 2.** Alternative encoding systems

| Classes of alternatives | Accessibility considerations | Downstream implications |
|---|---|---|
| Two-letter triplet codes | Simpler metabolism | Longer codons or fewer genetically encoded amino acids |
| Four-letter doublet codes | Simpler codes | Fewer genetically encoded amino acids |
| Quadruplet codes | Stronger anticodon binding | Potentially burdensome complexity (additional tRNA/aminoacyl tRNA synthetase pairs) |
| Punctuated codes (various) | Potentially strong codon binding/alignment mechanisms | Prevents large steps in sequence space via frameshift mechanism |
| Heterogeneous codon lengths | Less required uniformity | Irregularities constrain paths in sequence space |

support strong Watson-Crick pairing, have found extensive laboratory applications [34], and include plausible alternatives to nucleic acids from the perspectives of both biochemistry and evolution. To parallel the functional biology of nucleic acids, uncharged amide linkages could be complemented by ionized carboxylic acid or amine functional groups (to provide the requisite polyanionic or polycationic structures [35]), which are both chemically rich and ubiquitous in biology. Genetic systems based on peptide nucleic acids might well be more accessible than analogs of the terrestrial phosphate/sugar system.

In addition to alternative backbones, experimental work has identified a wide range of potential alternatives to the terrestrial set of nucleobases [36], some of which are compatible with terrestrial DNA and RNA polymerases [37] [38]. Among these are base pairs that have be used to expand the terrestrial genetic code from 4 to 6 letters [39] *in vitro.*

Terrestrial nucleobases pair via arrays of hydrogen bonds, but alternative pairing mechanisms exist. In particular, incorporation of at least one ionic pair (e.g., an amine and a carboxylic acid) could plausibly reduce metabolic complexity, strengthen binding, and enrich the chemical functionality of transcripts beyond that available in the terrestrial RNA world.

Because of the diversity of potential backbone and nucleobase chemistries, the frequency with which post-AGT evolution settles on terrestrial-like or alternative genetic chemistries is an open question, and is arguably low. The potential implications of specific alternative chemistries for subsequent evolutionary capacity is unclear, but the consequences are potentially large enough to substantially constrain evolutionary rates or paths (table 1).

## Alternative encoding systems

Strong uncertainty surrounds the joint development of ribosomes and the terrestrial triplet codon system [40]. Physical considerations suggest that triplet codes are themselves a product of evolution: triplet codon/anticodon pairs provide adequate specificity, but only weak binding, while longer codons would provide both ample specificity and more stable binding [41]. Longer codons are certainly possible: Modern ribosomes, evolved to support a triplet code, can translate 4-base [41, 42, 43] and even 5-base [44] codons. Accordingly, it has been argued that the most plausible path to ribosomal translation would start with longer codons, with the emergence of the modern triplet code requiring incremental reduction of codon size [41]. Traversing this path would, however, entail a sequence of changes in genetic encoding, and a system that froze with mixed-length encodings would be subject to a range of downstream evolutionary impediments

**Table 3.** Alternatives to translated genetic codes

| Classes of alternatives | Accessibility considerations | Downstream implications |
|---|---|---|
| Persistent RNA-world analogs | No strong GGT required | Sharply constrained chemical/structural basis for enzyme-like functionalities (a characteristic of modern ribozymes) |
| Rich transcripts | No tRNA or ribosomal machinery | Retention of codon nucleobases and backbone segments constrains product structures and lowers the density of encoded information per unit molecular weight |
| Transcript functionalization | Fully incremental development | Retention of codon-length backbone segments constrains structures and lowers the density of encoded information per unit molecular weight of product |

that includes ambiguity constraints on codon sequences and disruptive frame shifts induced by point mutations.

Punctuated codes (triplet codons separated by "commas") could potentially resolve problems of small-codon binding affinity while providing the putative advantages of triplet encodings, and would also provide a natural mechanism for aligning translation with reading frames (indeed, punctuation was once considered necessary for this purpose [45]). The advantages of punctuation, together with the weakness of constraints on the nature of "commas", suggest that there are many potential instantiations of punctuated codes, and that one or more of these may be more accessible than the terrestrial system of contiguous, unpunctuated triplet codons. The potential implications of punctuated codes for subsequent evolutionary rates are unclear but potentially significant. Augmentation of per-codon binding strength by punctuation would also enable the use of a shorter, simpler doublet code.

A potentially more severe constraint would be a genetic system locked into a simpler nucleobase system: As Crick observed, "anyone can see that the original nucleic acid may only have had two bases instead of four" [25]. It seems likely that a simpler, two-letter triplet code would be both more accessible and equally prone to freezing, and that the downstream effects on evolutionary capacity could be severe.

## Alternatives to translated genetic codes

The complexity and indirect nature of ribosomal translation suggests that GGTs to translational genetic systems may face strong barriers. An obvious hypothesis is that the persistence of an RNA (or RNA-analogue) world is a more common evolutionary path. The restricted chemical functionality of ribozymes, however, suggests that a persistent RNA world might support only biologies of low evolutionary capacity, perhaps encountering a ceiling on metabolic and cellular complexity (e.g., fewer metabolites, or no transition to the equivalent of eukaryotic cells). The potential existence of RNA analogues with greater chemical versatility (e.g., employing amine/carboxylic acid pairs, alternative nucleobases, or a more diverse set of nucleobases) introduces further uncertainties regarding potential evolutionary paths, as noted below.

There are, however, potential alternatives to both translation and RNA world analogues. For example, modern DNA/RNA genetic system illustrates a general principle, the use of a genetic polymer (DNA) to template a distinct polymer with greater structural and chemical functionality (RNA). Taking this functional-transcript principle further, a genetic system might employ a codon-by-codon transcription mechanism in which different transcript codons would bear different chemical functionality, yielding relatively rich, protein-like transcripts without employing ribosomes, sets of tRNA molecules, and complementary synthetases. Laboratories have constructed based-pairing polymers (PNAs with backbones bearing protein-like side-chains [46]) that exceed RNA in potential chemical functionality; further work has demonstrated that such polymers can be templated by DNA [47]. However, the retention of codon nucleobases and backbone segments in simple transcription-based systems would constrain product structures and lower the density of encoded information per unit molecular weight.

In another plausible class of non-translational alternatives, genetic sequences would rely on transcript functionalization, determining the structure of functionally rich polymers by sequence-directed enzymatic modification of a less functional transcript (perhaps similar or identical to the genetic polymer itself). In place of the complex and indirect mechanisms of ribosomal translation, we would find a set of incrementally developed enzyme analogues that recognise and bind to specific transcript sequences, directing diverse modifications of a structure that is initially as regular as RNA. In a systematic, unidirectional version of this class of schemes, enzyme or ribozyme analogues would bind specific coding sequences via anticodon-like complementarity and then modify upstream sites, leaving downstream coding sequences open for further steps of matching and upstream modification. As with rich-transcript systems, simple transcript-functionalization systems would constrain product structures and lower the density of encoded information per unit molecular weight. It is, however, easy to envision systems in which extraneous codon-derived backbone segments would be eliminated by operations analogous to exon removal by RNA splicing.[3]

## Summary: Alternatives systems and evolutionary capacity

To recap, we know that terrestrial evolution from prokaryotes to eukaryotes to metazoa to large-brained vertebrates required several steps that each unfolded on a billion-year time scale, a large fraction of the present age of the universe. We do not know what features of our biology determined even the order of magnitude of this time scale, but those features are presumably dependent on the specific nature of accessible microevolutionary transitions conditioned by genetic and metabolic mechanisms.

We also know that microevolutionary transitions in terrestrial evolution exploited a particular genetic system, one that employs sugar-phosphodiester nucleic acids to transmit information and accumulate genetic change, while producing functionally rich molecules through a mechanistically-distinct ribosomal translation system that employs a particular kind of uniform encoding with 2 base types and triplet codons. As discussed above, present knowledge of chemistry and molecular biology suggests a host of alternative genetic systems, several of which, if developed, would likely commit subsequent organisms to an evolutionary trajectory subject to a substantially lower capacity for the development of biological complexity, and yet are plausibly simpler and more evolutionarily accessible than our own. Considering rate alone, a log-factor of 5 impairment in capacity would place the emergence of complex life in such a system beyond the current cosmological time scale.

[3]Features of terrestrial molecular biology suggest that commitment to RNA-like genetic chemistries may impede the emergence of chemically-rich transcript-functionalization systems: Observed modifications to RNA backbones primarily serve regulatory or structural roles, and RNA nucleobase modifications, though more varied, are either minor or rare [48]. This circumstance can perhaps be explained (in part) by the difficulty of functionalizing charged phosphodiester linkages (and the consequent persistence of strong, structurally destabilizing charge-charge repulsion) together with the impoverished, single-hydroxyl chemical functionality of the backbone ribose moiety. Alternative genetic chemistries would not necessarily be subject to these chemical constraints; in particular, amide backbones charged by the ionization of easily functionalized (and neutralized) amine or carboxylic-acid groups would lend themselves to rich post-transcriptional modification.

It may or may not be the case that one or more of the universal yet evolutionarily contingent features of terrestrial genetic systems was essential to the rate and scope of terrestrial evolution. Accordingly, in assessing the current $\mathrm{LU}[f_i]$, it is of interest to consider the *scale of our uncertainty* regarding the prevalence of alternative biologies, considering both rates and ratios of the frequencies of alternative GGTs.

## Formulating models of GGT rates and ratios

As noted above, uncertainties regarding the frequencies of GGTs and their outcomes can be framed in at two ways: first, as transitions that occur at some rate per unit time in a pool of organisms, and second, as processes in which we factor out rates, populations, and time intervals, and consider instead the ratios of competing GGTs and their outcomes. Uncertainties in rates speak to the potential occurrence of a GGT against the background of a given genetic system; uncertainties in ratios speak to the potential occurrence of a GGT in the context of competing evolutionary paths.

### Rates, ratios, and the origin of large LUs

We find that log-broad uncertainties can arise through several mechanisms, some of which build on others. Taken together, they establish that log-broad uncertainties are by no means a special case, and that they can have large downward extents. The following mechanisms are not mutually exclusive, and we make no claim that they are collectively exhaustive.

### Thermodynamics, rates, and product ratios

Molecular processes are fundamental to molecular biology and the mechanisms underlying GGTs, and molecular processes easily give rise to log-broad distributions or parameters. For example, some reaction rates are fast, occurring on a molecular collisional time scale, while others are extraordinarily slow; for similar reasons, some reactions move toward an equilibrium in which almost all reactants are consumed to make products, while others would yield no molecules of product in a volume of reactants of astronomical scale.

To offer illustrative numbers regarding the thermodynamics of rates and equilibria, introducing an energy barrier equal to the free energy of formation of a single $CO_2$ molecule ($\Delta G > 390\,\mathrm{kJ\,mol^{-1}}$) would reduce the reaction rate along a chemical pathway by a factor of $\approx 10^{-65}$ at at $300\,\mathrm{K}$. In an example of relevance to biology (or models of abiogenesis), the free energy of peptide-bond hydrolysis in water is $\Delta G \approx 10\,\mathrm{kJ\,mol^{-1}}$ [49], hence a series of 50 peptide polymerization steps by would yield a product/reactant ratio $< 10^{-85}$. In both instances, log-large ratios result from expressions containing factors of the form $\exp(-\Delta G/kT)$.

### Combinatorics and transition rates

The general structure of the Levinthal protein-folding paradox is again relevant. In the absence of convergent, funnel-like stabilization of intermediate pathway states (that is, a path with generally declining free energy), complex systems that require the assembly of a particular configuration of many parts are subject to the equivalent of the Levinthal paradox, which in thermodynamic terms describes systems with large entropic transition-state barriers. Once again, log-broad ratios emerge: For systems characterized by $N$ binary degrees of freedom, transition rates to any particular state decline as $2^{-N}$. Genetic transitions that explore a large state space present a qualitatively similar picture, with differential fitness along paths playing a role analogous to differences in energy.

### Intermediate-fitness barriers

In an evolutionary context, a path to a state with long-term (or even short term) advantages will be inaccessible if the path would entail a interval of strong or prolonged competitive

disadvantage. The discussion of codon substitution below gives a concrete example in terrestrial biology.

## Race-outcome ratios

Models of races between alternative paths can also yield large outcome ratios. In a Poisson race model there is a sequence of $K_i$ discrete steps that must occur for each outcome $i$ to happen, with a $1/\lambda_i$ exponentially distributed waiting time for each step. The ratio of outcome 1 to 2 occurring is $R = p_1/(1-p_1)$ where $p_1 = \mathrm{betacdf}(\lambda_1/(\lambda_1+\lambda_2), K_1, K_2)$. $R \propto (\lambda_2/\lambda_1)^{-K_1}$ for large $\lambda_2/\lambda_1$ (branch 2 is fast compared to branch 1), and $R \propto (\lambda_2/\lambda_1)^{-K_2}$ for small $\lambda_2/\lambda_1$ (branch 1 is faster). A given log-ratio is hence *multiplied* by the relevant $K_i$. For a GGT this could potentially be a non-trivially large integer[4].

## Branching-path ratios

Thermodynamic, combinatorial, and race-outcome considerations suggest the ease with which large ratios can emerge in molecular and evolutionary systems, but even modest ratios can compound if they describe alternative steps on a branching path. A discussion below outlines a model in which the path to a high-capacity genetic system requires a series of branching choices (between codons of length 3 and 4), each of which favors the off-path alternative by a ratio $R_{step}$. Success in following such a path will scale as $R_{step}^{N_{steps}}$, which can easily be $> 100^{50}$. In the above taxonomy, thermodynamic, combinatorial, and intermediate-fitness considerations pertain to what are conceptually single-step processes, while race-outcome and branching-path ratios can be modeled as the results of multi-step processes in which each step is subject to thermodynamic, combinatorial, and fitness considerations.

## GGT models and $LU$ values

Without implying a sharp demarcation between biological systems before and after a particular GGT, is natural to describe GGTs as biological events that occur in a population of reproducing organisms at some (uncertain) rate per reproductive cycle. In this model of a GGT, time and population play roles parallel to those of time and substrate volume in AGT models.

Unlike AGT models, however, GGT models must take account of the potential displacement (or preclusion) of a genetic system $G_i$ by a more-competitive successor $G_j$. For every transition $G_i \rightarrow G_j$, the emergence of a strongly competitive system $G_j$ precludes alternative transitions $G_i \rightarrow G_k$ and potential systems downstream from $G_k$ (without loss of relevant generality, we can define GGTs as transitions to strongly competitive systems in this sense). In terrestrial history, the GGT that ended the RNA world, $G_{RNAworld} \rightarrow G_{modern}$, both displaced $G_{RNAworld}$ and precluded potential alternative transitions $G_{RNAworld} \rightarrow G_{unknown}$; conversely any of a range of potential transitions $G_{RNAworld} \rightarrow G_{unknown-}$ would have precluded the emergence of the modern terrestrial genetic system (or on-path alternatives).

More generally, we can consider a family of evolutionary paths through a set of systems $\{G^+\} \cup \{G^-\}$, in which systems $G_{i+} \in \{G^+\}$ and $G_{j-} \in \{G^-\}$ are (respectively) systems that are on and off paths that potentially lead to complex life. In other words, transitions $GGT_{i+,j+}$ are on-path, transitions $GGT_{i+,j-}$ and $GGT_{i-,j-}$ are off-path, and transitions $G_{i-} \rightarrow G_{j+}$ by definition do not occur (or equivalently, occur with contextually negligible magnitudes). We can further distinguish terminal genetic systems $G^T \in \{G^{T+}\} \cup \{G^{T-}\}$ as those that persisted until the present cosmological time.

AGTs may also be of different kinds with different downstream consequences for evolutionary capacity. To place this possibility in a uniform framework, we can represent prebiotic environments as null, on-path genetic systems $G_{0+}$, and alternative AGTs as elements of a set $GGT_{0,i+} \cup GGT_{0,i-}$.

[4]The model assumes constant rates $\lambda_i$; in reality different steps in a GGT will likely have different speeds. For our purposes the full sequence of steps may be compressed to a roughly equivalent effective sequence with constant rates, typically with $K_i$ corresponding to the number of states with minimal rates.

A fine-grained model would distinguish every mapping from codons to amino acids as a distinct genetic system, but a model with this level of detail has no use in the present context. We will instead consider a simplified coarse-grained picture, defining classes of genetic systems by their evolutionary capacity ($G^-$ or $G^+$), and by their position in a coarse-grained picture of a sequence of genetic systems ($G_1^+, G_1^-; G_2^+, G_2^-; \ldots$) along a path leading through a series of branch points to $G^{T+}$ and $G^{T-}$ systems.

We have seen that multiple mechanisms can contribute to log-broad uncertainties in outcome ratios, so this picture, it is natural to think in terms of ratios of competing transitions, $\log(\Pr(GGT_{i-1,i+}) / \Pr(GGT_{i-1,i-})) = \mathrm{LR}^{+/-}[G_i]$. We argue that any of several branch points $i$ have evidently large values of $\mathrm{LU}^{+/-}$ that extend to small values $\mathrm{LR}^{+/-}$.

The probability that a particular genetic system $G$ is an element of the terminal set $G^T$ will depend on the transition rates of potential subsequent GGTs relative to available time intervals (e.g., gigayears). The terrestrial example suggests that $G^T$ systems typically arise early on a planetary time scale as genetic systems become consolidated ("freeze") by consuming coding capacity and metabolic resources, riving rise to complex regulatory and metabolic systems that both support and exploit the increasingly entrenched system.

### Potentially critical GGT branch points

Questions regarding the emergence of the terrestrial RNA world its successors provide a relatively concrete context for discussing the range of plausible $\mathrm{LR}^{+/-}[G_i]$ values, with the development of translation-based (broadly, ribosomal) systems as a central theme. Decades ago, Crick observed that "The origin of protein synthesis is a notoriously difficult problem," [50] and the years since then have produced many plausible proposals, but no widely-accepted model for the *initial emergence* of the machinery of a translation-based genetic system [40, 41, 51]. Accordingly, the accessibility of GGTs that lead from an RNA world to ribosome-like translation is an open question. And, quite naturally, neither the accessibility of translational systems from alternative RNA-like genetic systems, nor the accessibility of competing translational or non-translational systems, has played a substantial role in studies of the origin and development of terrestrial life.

## Non-equivalent XNA alternatives

It would be unsurprising to find that GGTs leading to alternative RNA-like genetic chemistries (see candidates in Table 1) dominate evolutionary paths. Note that systems with different chemistries will have different metabolic requirements; if these differ in complexity, simpler systems maybe favored by large ratios, in which potential thermodynamic, combinatorial, race-outcome, and branching-path considerations are all salient. It would be unsurprising to find that a large GGT-ratio favors simpler RNA-like structures that entail downstream constraints on evolutionary capacity.

Conversely, if the chemical complexity of RNA-like molecules can increase incrementally without encountering fitness barriers, it would be unsurprising to find that RNA-like worlds emerge in which transcripts with extensive chemical functionality provide direct competitive advantages, yet impede the emergence of a small, tractable sets of codons. Race-outcome and branching-path considerations then easily support arguments for large GGT-ratios that favor the elaboration of transcript-based biological systems over the emergence of indirect, translational genetic systems.

## Rich-transcript biologies

Competition between genetic systems based on translational and non-translational (transcriptional) encodings of functionally rich products can be formulated as a race model in which the steps are increments (e.g., in metabolic function) toward the threshold of a relatively rich, subsequently consolidated translational or transcriptional genetic system. The winner of the

race is the translational or transcriptional system that first achieves a strong advantage in the sense that selective pressures favor shifting coding and metabolic resources toward the elaboration of that system and displacement of its alternative. The greater complexity of translational systems suggests that the threshold number of steps is much lower for transcriptional systems, and plausible race models yield large GGT-ratios in favor of the latter.

## Alternative translational systems

As discussed above, there are many potential alternative versions to the terrestrial system of contiguous 4-letter triplet codons. Moreover, as discussed above, there is substantial reason to think that the terrestrial system is derived from an earlier system in which some or all codons were longer (e.g., quadruplets), and then incrementally shortened to the yield the current system. In a model of incremental codon addition, one might find that quadruplet codons were favored over triplet codons by a substantial factor (e.g., $> 1000$) in a branching-path process; after 20 codon assignments, a 4-base or mixed-length system would be favored by a factor $> 1000^{20}$.

Terrestrial history suggests that reduction of a quadruplet or mixed-length system to a uniform triplet system would be very unlikely. The "frozen accident" of specific triplet codon assignments [52] was not, in fact, completely frozen. To date, biological studies have identified divergences from the canonical genetic code in $\approx 40$ lineages, but each divergence reassigns only a single codon. In the terrestrial history of $\approx 10^{40}$ reproduction events ($1.7 \times 10^{30}\ \mathrm{yr}^{-1}$ [53]), this amounts to a single-codon GGT rate of $\approx 10^{-38}$.

In a uniform code, single codon reassignments constitute point mutations in every protein whose gene contains that codon, hence abrupt codon reassignment would typically be lethal. And abrupt reduction in the length of a codon would result in a yet more consistently lethal frameshift mutation in every such protein. In a simple model of abrupt, uncompensated transitions, this difficulty is an ideal model of an intermediate-fitness barrier: The benefits of a step would result from long-term evolutionary potential, but lethality precludes short-term survival.

It is natural to expect that nonuniform codes, no matter how accessible they might be initially, would suffer from handicaps with respect to downstream evolutionary capacity; according to the argument above, it would be unsurprising to find that such codes were both overwhelmingly common and effectively impossible to displace, and that they consistently slow the pace of evolutionary change by a factor $> 10$. (For a contrary argument, see Baranov [41], who suggests that translation began with quadruplet codons, but underwent rapid codon size reduction to a triplet code by a facile, convergent pathway.)

In general, the extraordinarily low rate of successful post-LUCA GGTs, even at the microscale of single-codon reassignments, suggests large downward uncertainty regarding transition rates for more substantial GGTs on the path to a LUCA-organisms in alternative planetary biologies. It would be unsurprising to find that strong lock-in is a common property of diverse genetic systems.

## Unknown competing paths

Similarly, we can have no confidence that nucleic-acid-like genetic systems are requisite for effective living systems, where "effective" is defined by the capacity to consume the substrate for AGTs or early life, precluding alternative AGTs. As with other GGTs, the nature of the physical processes involved and our limited knowledge call for assigning large values of $LU$ (extending to low values of LR underscore (+/âĂŞ)) to competing classes of AGTs. It may also be that pathways to high-capacity life consistently (with high LR) pass through non-nucleic-acid-like systems, which would point to a subsequent, large-LU GGT to an RNA or XNA system (note that this prospect undercuts potential arguments that life must be rare because of difficulties in envisioning abiogenesis via RNA [4]). Because the alternatives and uncertainties outlined above involve unknown processes leading to systems of unknown kinds, there is little more to be said here.

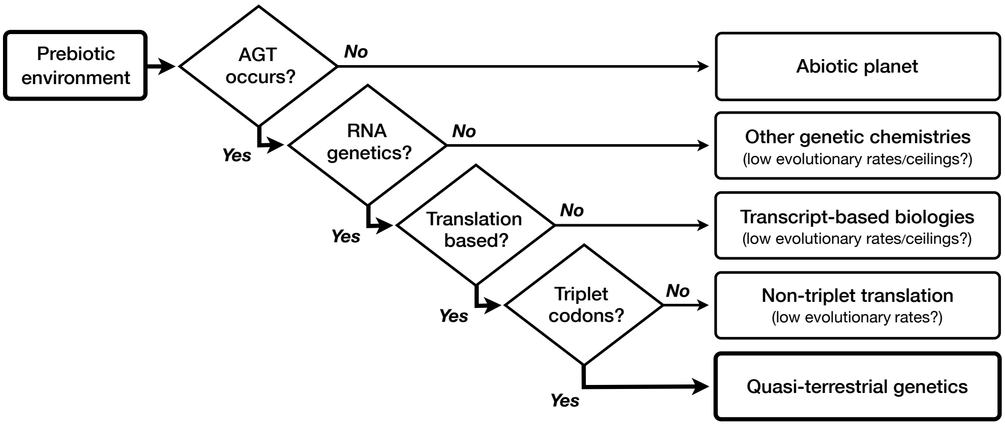


**Figure 1.** A schematic diagram of potential AGT and GGT branches with aggregated states and transitions. At each branch point, outcome ratios are weakly constrained, with $\mathrm{LU}$ values arguably $> 100$.

## Summary and conclusion

We have identified mechanisms that can naturally lead to large LU values for the rates and outcome-ratios of processes involving transitions in complex systems. From a molecular perspective of particular relevance to AGTs, potential adverse energetic or entropic requirements can reduce transition rates and product concentrations by factors with low (e.g., $< -50$) LR values. Similarly, models of GGTs easily yield large values of $LU$ and low LR; simple instances are Poisson races between paths with differing numbers of requisite steps, and branching paths in which a particular outcome requires a series of low-probability choices. Finally, from the perspective of evolutionary paths, steps that lead to low-fitness intermediates can be effectively blocked.

Uncertainty regarding potential AGT processes has been extensively discussed in literature on the origin of life and prevalence of intelligent life in the universe. Here, modeling AGT processes as physical processes characterized by volumetric rate constants, and show that, given present information, it would require implausible knowledge claims to argue for values of log uncertainty and the downward extent of outcome ratios are less than several hundred.

Uncertainty regarding potential GGT processes has been less explored, and we discuss potential branching points in which outcomes could either enable or preclude the evolution of complex life. The salient examples can be grouped into three broad classes of alternatives to the terrestrial path: XNA biologies that differ in critical ways from the terrestrial RNA-world biology; rich-transcript biologies that elaborate and entrench alternative mechanisms for extending an RNA/XNA world with more nearly protein-like functional molecules, and variants of translational systems that would employ irregular or other potentially impaired encodings of amino acids. A final, very general possibility, is the potential for AGT processes to lead to unknown biologies of unknown kinds. Each of these alternatives is plausible (which is to say, consistent with present knowledge), and the first three are more than plausible, in that relatively concrete and moderately persuasive arguments can be constructed for their likelihood.

It should be noted that the literature on the origin of terrestrial life seeks to identify paths of maximum plausibility; this an appropriate goal, but does not directly address the questions of uncertainty raised here, particularly those that involve alternatives to terrestrial genetic systems. By contrast, to argue for confidence that the distribution over $f_l f_i$ has no log-broad tail extending to low values would require strong knowledge claims regarding $\mathrm{LR}^{+/-}$ and $\mathrm{LU}^{+/-}$ parameters

not only for AGT events, but for a series of subsequent potential and actual GGTs. A conjunction of these knowledge claims would seem difficult to support.[5]





## References


1 David S Spiegel and Edwin L Turner. Bayesian analysis of the astrobiological implications of lifeâĂŹs early emergence on earth. *Proceedings of the National Academy of Sciences*, 109(2): 395–400, 2012.

2 Kepa Ruiz-Mirazo, Carlos Briones, and Andrés de la Escosura. Prebiotic systems chemistry: new perspectives for the origins of life. *Chem. Rev*, 114(1):285–366, 2014.

3 Michael P Robertson and Gerald F Joyce. The origins of the rna world. *Cold Spring Harbor perspectives in biology*, 4(5):a003608, 2012.

4 Harold S Bernhardt. The rna world hypothesis: the worst theory of the early evolution of life (except for all the others) a. *Biology direct*, 7(1):1, 2012.

5 Thomas M McCollom. Miller-urey and beyond: what have we learned about prebiotic organic synthesis reactions in the past 60 years? *Annual Review of Earth and Planetary Sciences*, 41: 207–229, 2013.

6 Addy Pross. Physical organic chemistry and the origin of life problem: A personal perspective. *Israel Journal of Chemistry*, 56(1):83–88, 2016.

7 John D Sutherland. The origin of lifeâĂŤout of the blue. *Angewandte Chemie International Edition*, 55(1):104–121, 2016.

8 Pier Luigi Luisi. Chemistry constraints on the origin of life. *Israel Journal of Chemistry*, 55(8): 906–918, 2015.

9 Stuart A Kauffman. Autocatalytic sets of proteins. *Journal of theoretical biology*, 119(1):1–24, 1986.

10 Giovanna Costanzo, Samanta Pino, Fabiana Ciciriello, and Ernesto Di Mauro. Generation of long rna chains in water. *Journal of Biological Chemistry*, 284(48):33206–33216, 2009.

11 Samanta Pino, Fabiana Ciciriello, Giovanna Costanzo, and Ernesto Di Mauro. Nonenzymatic rna ligation in water. *Journal of Biological Chemistry*, 283(52):36494–36503, 2008.

12 Paul G Higgs and Niles Lehman. The rna world: molecular cooperation at the origins of life. *Nature Reviews Genetics*, 16(1):7–17, 2015.

13 Jean-François Lambert. Adsorption and polymerization of amino acids on mineral surfaces: a review. *Origins of Life and Evolution of Biospheres*, 38(3):211–242, 2008.

14 Sandra Pizzarello. The chemistry of life's origin: A carbonaceous meteorite perspective. *Accounts of Chemical Research*, 39(4):231–237, 2006.

15 K Hans Wedepohl. The composition of the continental crust. *Geochimica et cosmochimica Acta*, 59(7):1217–1232, 1995.

16 Paul C Lauterbur. The spontaneous development of biology from chemistry. *Astrobiology*, 8 (1):3–8, 2008.

17 Guenter Wulff. Molecular imprinting in cross-linked materials with the aid of molecular templatesâĂŤa way towards artificial antibodies. *Angewandte Chemie International Edition in English*, 34(17):1812–1832, 1995.

18 Lei Ye and Klaus Mosbach. Molecular imprinting: synthetic materials as substitutes for biological antibodies and receptorsâĂă. *Chemistry of Materials*, 20(3):859–868, 2008.

19 Masahiro Yoshida, Yasuo Hatate, Kazuya Uezu, Masahiro Goto, and Shintaro Furusaki. Chiral-recognition polymer prepared by surface molecular imprinting technique. *Colloids and Surfaces A: Physicochemical and Engineering Aspects*, 169(1):259–269, 2000.

20 Cyrus Levinthal. Are there pathways for protein folding. *J. Chim. phys*, 65(1):44–45, 1968.

21 Robert Zwanzig, Attila Szabo, and Biman Bagchi. Levinthal's paradox. *Proceedings of the National Academy of Sciences*, 89(1):20–22, 1992.


[5]Observations of extraterrestrial biospheres would strongly update estimates of AGT probabilities, but would only weakly update $\mathrm{LU}^{+/-}$ for AGTs on pathways to organisms with high evolutionary capacity. Because the evolution of organisms with even a small fraction of the metabolic competence of terrestrial prokaryotes could enable photosynthesis and transform chemistry on a planetary scale, log-broad uncertainties in $\mathrm{LU}[f_L]$ would remain.

22 Ken A Dill, Hue Sun Chan, et al. From levinthal to pathways to funnels. *Nature structural biology*, 4(1):10–19, 1997.

23 J Doyne Farmer, Stuart A Kauffman, and Norman H Packard. Autocatalytic replication of polymers. *Physica D: Nonlinear Phenomena*, 22(1):50–67, 1986.

24 David P Horning and Gerald F Joyce. Amplification of rna by an rna polymerase ribozyme. *Proceedings of the National Academy of Sciences*, page 201610103, 2016.

25 Francis HC Crick. The genetic codeâĂŤyesterday, today, and tomorrow. In *Cold Spring Harbor symposia on quantitative biology*, volume 31, pages 3–9. Cold Spring Harbor Laboratory Press, 1966.

26 Albert Eschenmoser. Chemical etiology of nucleic acid structure. *Science*, 284(5423):2118–2124, 1999.

27 Lilu Zhang, Adam Peritz, and Eric Meggers. A simple glycol nucleic acid. *Journal of the American Chemical Society*, 127(12):4174–4175, 2005.

28 Mark K Schlegel, Lars-Oliver Essen, and Eric Meggers. Duplex structure of a minimal nucleic acid. *Journal of the American Chemical Society*, 130(26):8158–8159, 2008.

29 Jeremy Bailey. Chirality and the origin of life. *Acta Astronautica*, 46(10):627–631, 2000.

30 Aaron E Engelhart and Nicholas V Hud. Primitive genetic polymers. *Cold Spring Harbor perspectives in biology*, 2(12):a002196, 2010.

31 Phaneendrasai Karri, Venkateshwarlu Punna, Keunsoo Kim, and Ramanarayanan Krishnamurthy. Base-pairing properties of a structural isomer of glycerol nucleic acid. *Angewandte Chemie*, 125(22):5952–5956, 2013.

32 Vitor B Pinheiro and Philipp Holliger. The xna world: progress towards replication and evolution of synthetic genetic polymers. *Current opinion in chemical biology*, 16(3):245–252, 2012.

33 Michael Egholm, Ole Buchardt, Peter E Nielsen, and Rolf H Berg. Peptide nucleic acids (pna). oligonucleotide analogs with an achiral peptide backbone. *Journal of the American Chemical Society*, 114(5):1895–1897, 1992.

34 Peter E Nielsen, Michael Egholm, et al. An introduction to peptide nucleic acid. *Curr Issues Mol Biol*, 1(1-2):89–104, 1999.

35 Steven A Benner, Zunyi Yang, and Fei Chen. Synthetic biology, tinkering biology, and artificial biology. what are we learning? *Comptes Rendus Chimie*, 14(4):372–387, 2011.

36 Andro C Rios and Yitzhak Tor. On the origin of the canonical nucleobases: An assessment of selection pressures across chemical and early biological evolution. *Israel journal of chemistry*, 53 (6-7):469–483, 2013.

37 Daniel H Appella. Non-natural nucleic acids for synthetic biology. *Current opinion in chemical biology*, 13(5):687–696, 2009.

38 Emily M Harcourt and Eric T Kool. Designer bases, base pairs, and genetic sets: biochemical and biological activity. 2014.

39 Ichiro Hirao, Tsuneo Mitsui, Michiko Kimoto, and Shigeyuki Yokoyama. An efficient unnatural base pair for pcr amplification. *Journal of the American Chemical Society*, 129(50): 15549–15555, 2007.

40 David W Morgens. The protein invasion: a broad review on the origin of the translational system. *Journal of molecular evolution*, 77(4):185–196, 2013.

41 Pavel V Baranov, Maxime Venin, and Gregory Provan. Codon size reduction as the origin of the triplet genetic code. *PLoS One*, 4(5):e5708, 2009.

42 Takahiro Hohsaka and Masahiko Sisido. Incorporation of non-natural amino acids into proteins. *Current opinion in chemical biology*, 6(6):809–815, 2002.

43 Wei Niu, Peter G Schultz, and Jiantao Guo. An expanded genetic code in mammalian cells with a functional quadruplet codon. *ACS chemical biology*, 8(7):1640–1645, 2013.

44 Takahiro Hohsaka, Yuki Ashizuka, Hikaru Taira, Hiroshi Murakami, and Masahiko Sisido. Incorporation of nonnatural amino acids into proteins by using various four-base codons in an escherichia coli in vitro translation system. *Biochemistry*, 40(37):11060–11064, 2001.

45 J Claude Bennett and William J Dreyer. Genetic coding for protein structure. *Annual review of biochemistry*, 33(1):205–234, 1964.

46 Peter E Nielsen and Gerald Haaima. Peptide nucleic acid (pna). a dna mimic with a pseudopeptide backbone. *Chemical society reviews*, 26(2):73–78, 1997.
47 Ralph E Kleiner, Yevgeny Brudno, Michael E Birnbaum, and David R Liu. Dna-templated polymerization of side-chain-functionalized peptide nucleic acid aldehydes. *Journal of the American Chemical Society*, 130(14):4646–4659, 2008.
48 Magdalena A Machnicka, Kaja Milanowska, Okan Osman Oglou, Elzbieta Purta, Malgorzata Kurkowska, Anna Olchowik, Witold Januszewski, Sebastian Kalinowski, Stanislaw Dunin-Horkawicz, Kristian M Rother, et al. Modomics: a database of rna modification pathwaysâĂŤ2012 update. *Nucleic acids research*, page gks1007, 2012.
49 R Bruce Martin. Free energies and equilibria of peptide bond hydrolysis and formation. *Biopolymers*, 45(5):351–353, 1998.
50 FHC Crick, S Brenner, A Klug, and G Pieczenik. A speculation on the origin of protein synthesis. *Origins of life*, 7(4):389–397, 1976.
51 George E Fox. Origin and evolution of the ribosome. *Cold Spring Harbor perspectives in biology*, 2(9):a003483, 2010.
52 Francis HC Crick. The origin of the genetic code. *Journal of molecular biology*, 38(3):367–379, 1968.
53 William B Whitman, David C Coleman, and William J Wiebe. Prokaryotes: the unseen majority. *Proceedings of the National Academy of Sciences*, 95(12):6578–6583, 1998.
