# Supplementary material for: Dissolving the Fermi Paradox
Source: arXiv:1806.02404 ancillary file (2018-06-06)
Supplement: Supplementary file 2 [file supplement-ii-effects.pdf]

PROCEEDINGS A

rspa.royalsocietypublishing.org

Research

Article submitted to journal

# Supplement II: Effects of different scenarios on the results

Anders Sandberg[1], Eric Drexler[1] and Toby Ord[1]

[1]Future of Humanity Institute

© The Authors. Published by the Royal Society under the terms of the Creative Commons Attribution License http://creativecommons.org/licenses/by/4.0/, which permits unrestricted use, provided the original author and source are credited.

THE ROYAL SOCIETY
PUBLISHING

## Synthetic data variations

Our conclusions are robust with respect to choice of distributions and their means, as long as at least one distribution has a large log-uncertainty.

### Strong knowledge of all parameters but one

Figure 1 demonstrates the effect of being certain about all input parameters save $f_l$, showing that the effect of its broad uncertainty alone is enough to drive the conclusions of the paper.

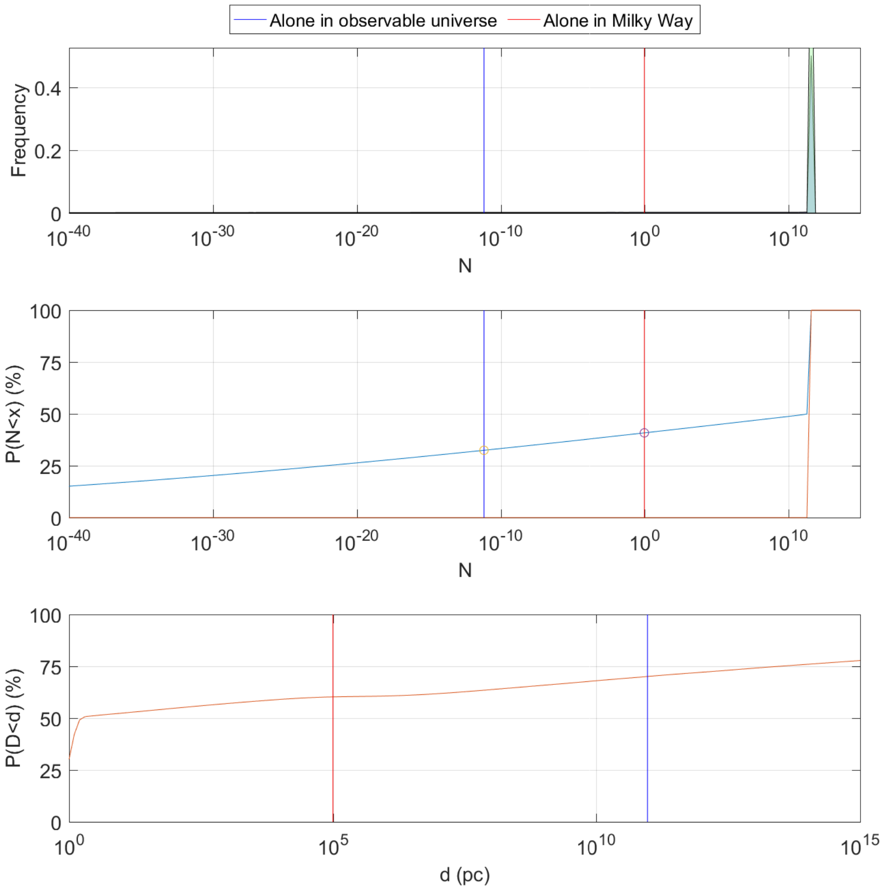


**Figure 1.** Effect of placing all parameters except $f_l$ at their most optimistic values found in the literature and reducing their uncertainty to zero. The effect of the broad life uncertainty still dissolves the Fermi paradox.

## Uniform parameters

The parameter distributions used in the rest of the paper have been log-uniform, implying a power-law probability distribution assigning more probability density to low values than high. Replacing them with uniform distributions with the same range does not change the qualitative

outcome significantly (figure 2): while this produces a very optimistic mean and median $N$ there is still a high probability of being alone.

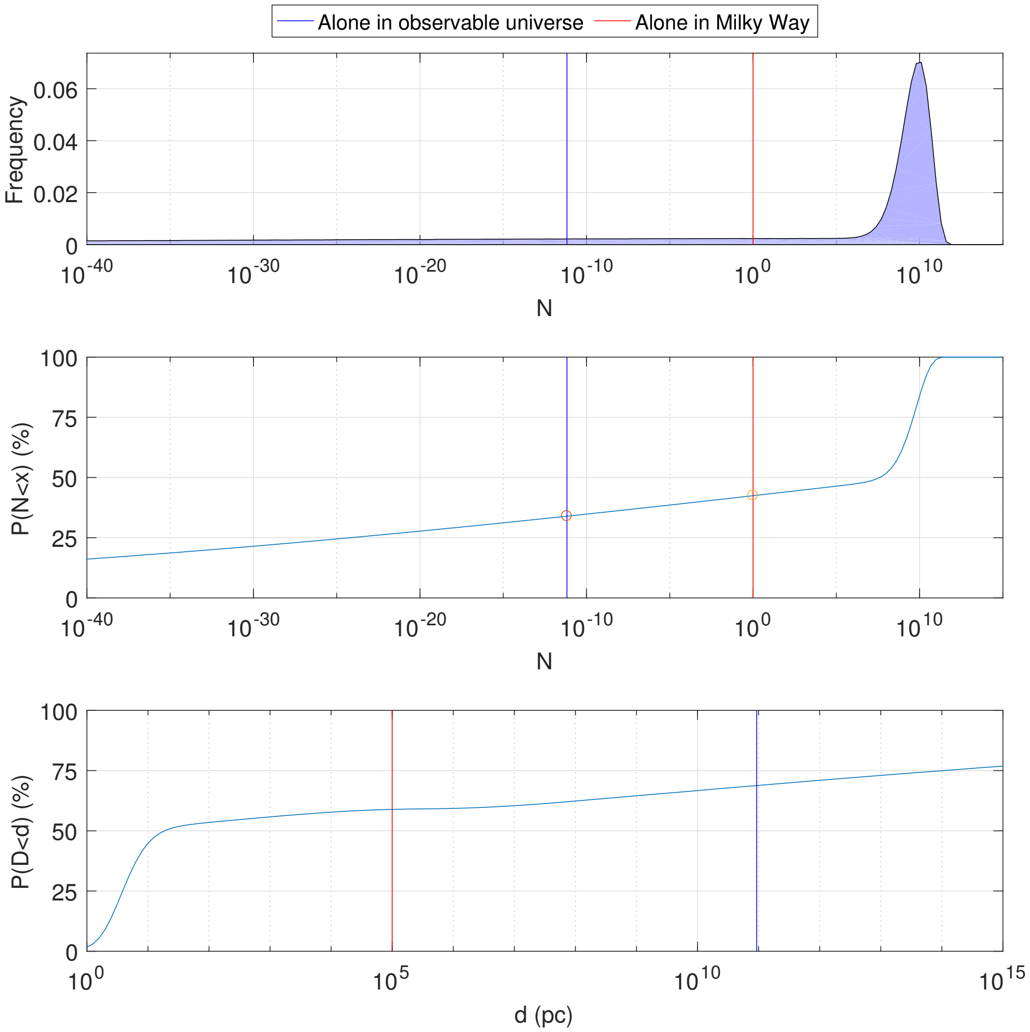


**Figure 2.** Effect of uniform distribution of all parameters except $f_l$.

## Equal uncertainty $f_l$ and $f_i$

The main model did not include the extra uncertainty in $f_i$ due to genetic coding systems with low evolutionary capacity; making $f_i$ distributed as $f_l$ with an underlying lognormal rate distribution strengthens the low-probability tail (figure 3).

## Fermi observations

The "Fermi observation" that we have not seen any evidence for ETI so far acts as a weak update on the distribution of $N$ and the parameters of the Drake equation.

As noted in the main text, the Fermi observation leads to an update of our credence distribution of $N$ as per BayesâĂŹ rule: $\Pr[N|\neg D] = \Pr[\neg D|N]\Pr[N]/\Pr[\neg D]$, where $\neg D$ denotes no

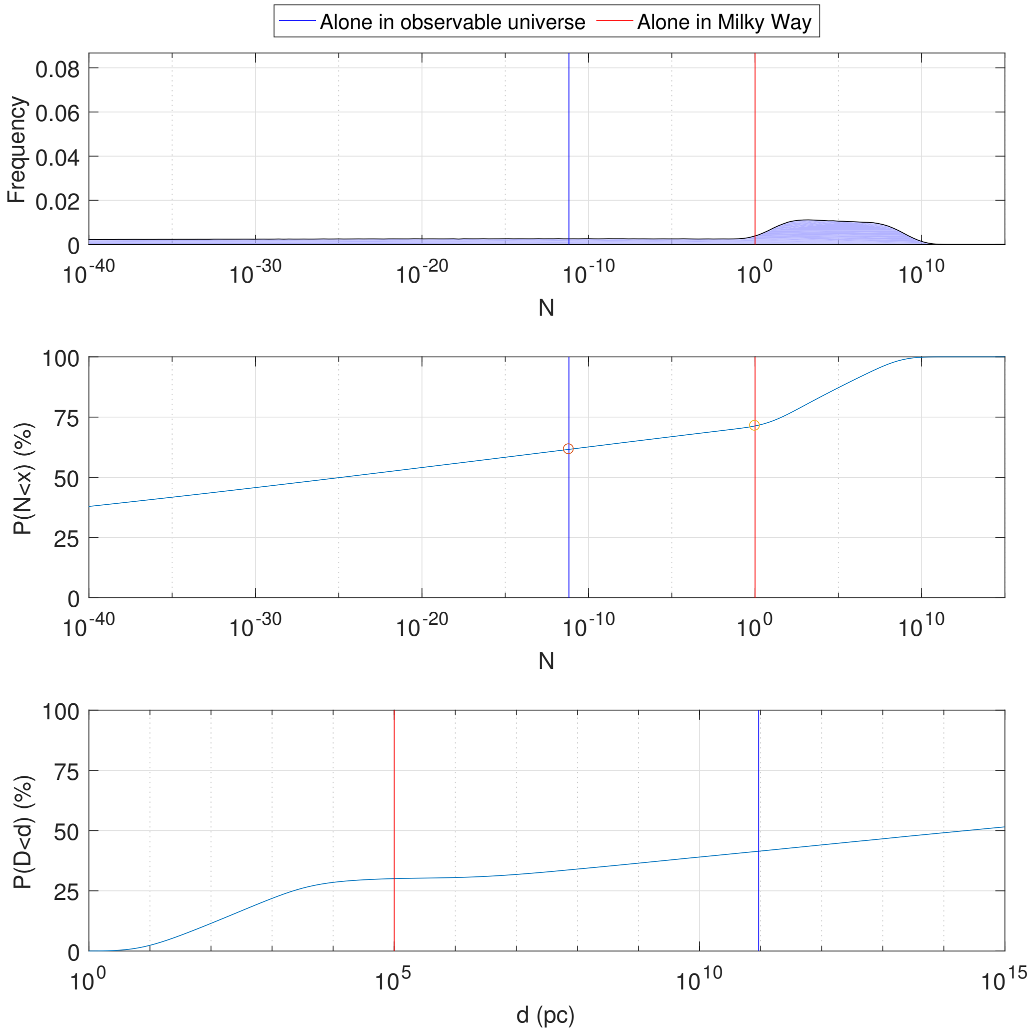


**Figure 3.** Effect of broad distribution of $f_i$.

detection. In the following we analyse different versions of the observation and the implied $\Pr[\neg D|N]$ term.

## Random sampling

If the observation is that out of $K$ sampled stars none have have a civilization, then

$$\Pr[\neg D|N,K] = (1-(N/N_{MW}))^K.$$

The effect is relatively mild, since the number of stars that needs to be sampled needs to be significant compared to the number of stars in the galaxy (figure 4).

## Spatial Poisson model

If the observation is that there is no civilization closer than some detection distance $d$,

$$\Pr[\neg D|N,d] = 1 - e^{-4\pi(N/V_{MW})d^3/3}$$

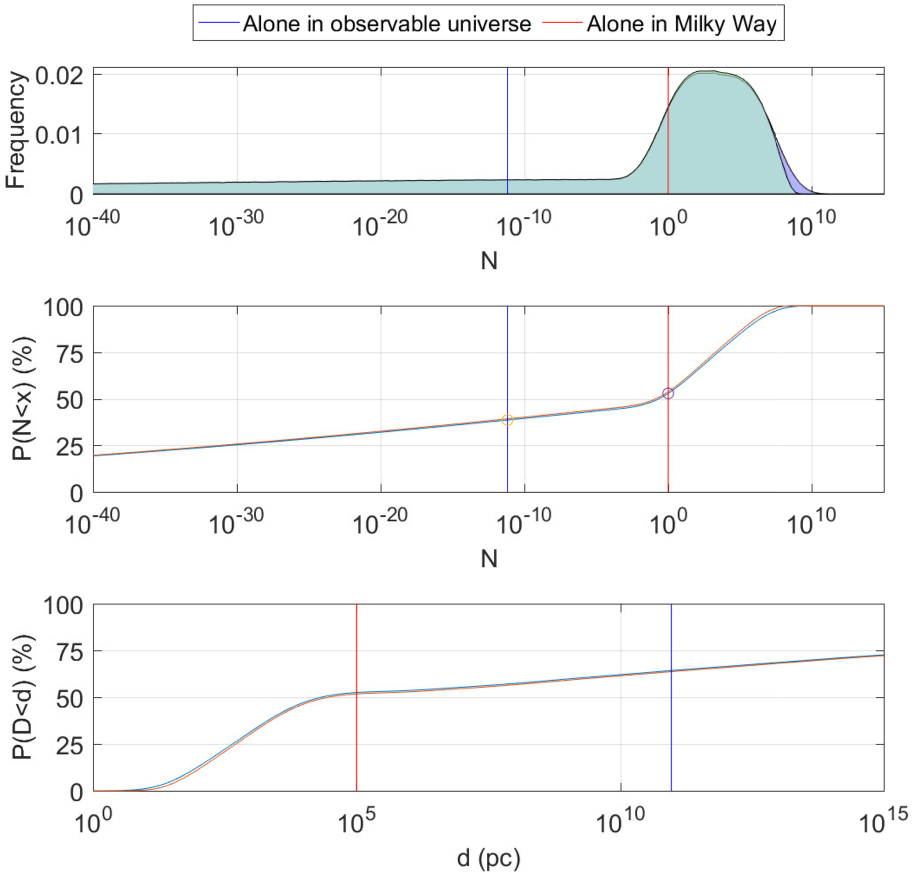


**Figure 4.** Effect of random sampling update of the Fermi observation, $K = 1000$.

where $V_{MW}$ denotes the volume of the Milky Way[1].

The effect is stronger on the positive tail than the random sampling update (figure 5).

## Cut-off factor

A very crude model of the Fermi observation is to assume that it corresponds to a factor $p_{fail}$ lowered probability of $N > N_0$. Here $P_{fail}$ corresponds to the possibility that for some reason we fail to detect even a teeming galaxy.

This conceptually corresponds to a simple observation that there cannot be large number of current civilizations, tempered by the possibility of either our observation failure or explanations of the Fermi paradox such as the "zoo hypothesis" or strong cultural convergence towards being hard to detect.

The effect is a step-wise reduction, leaving the lower tail invariant (figure 6). Changing the location of the cut-off affects the distribution of the parameters to different degrees (figure 7), with a stronger reaction from the more uncertain ones.

[1]This model is inaccurate for large $d$ since it presupposes a uniform star density, but since observable $d$ currently are far smaller than the galactic disc this is not a major issue

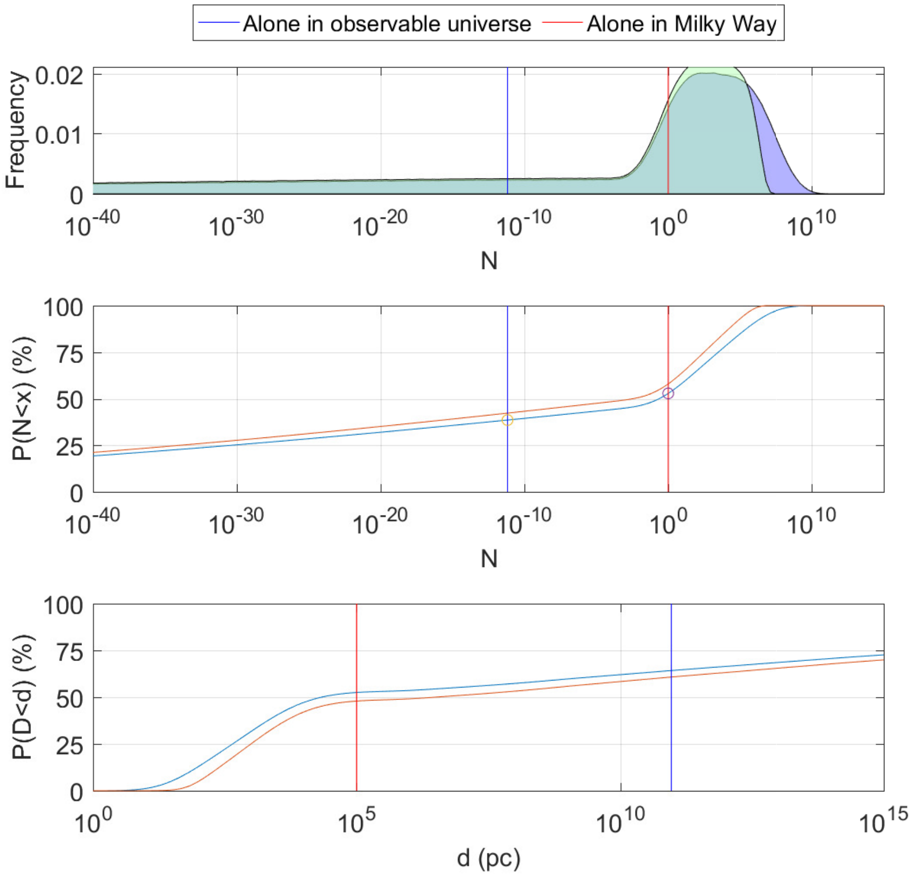


**Figure 5.** Effect of spatial poisson update, no civilization closer than $d = 18\,\mathrm{pc}$.

## Interstellar settlement models

Interstellar settlement models pose a conceptual problem to the Drake equation framework since it implicitly assumes a steady-state density of ETI in the galaxy. Given that an expanding civilization is unlikely to go extinct synchronously, interstellar settlement models imply that for civilizations colonizing the Milky Way $L$ must be larger than the colonization timescale (requiring a constraint on feasible $L$) or that the galaxy becomes permanently settled.

A way of deriving an update factor $\Pr[\neg D|N]$ in these cases is to model what fraction of spacetime that is not settled, assuming humanity is not in it.

The simplest model of interstellar settlement assumes that ETI spreads instantly in the galaxy ("swift expansion"): as long as there is at least one civilization extant it is incompatible with the Fermi observation. Placing this in a stochastic framework and treating the galaxy as a Poisson process,

$$\Pr[\neg D|N,d] = e^{-N}.$$

The second simplest model ("slow expansion") is, assuming a settlement timescale $T$ and civilization longevity $L$ where the galaxy is either empty or we are in an as-yet uncolonized

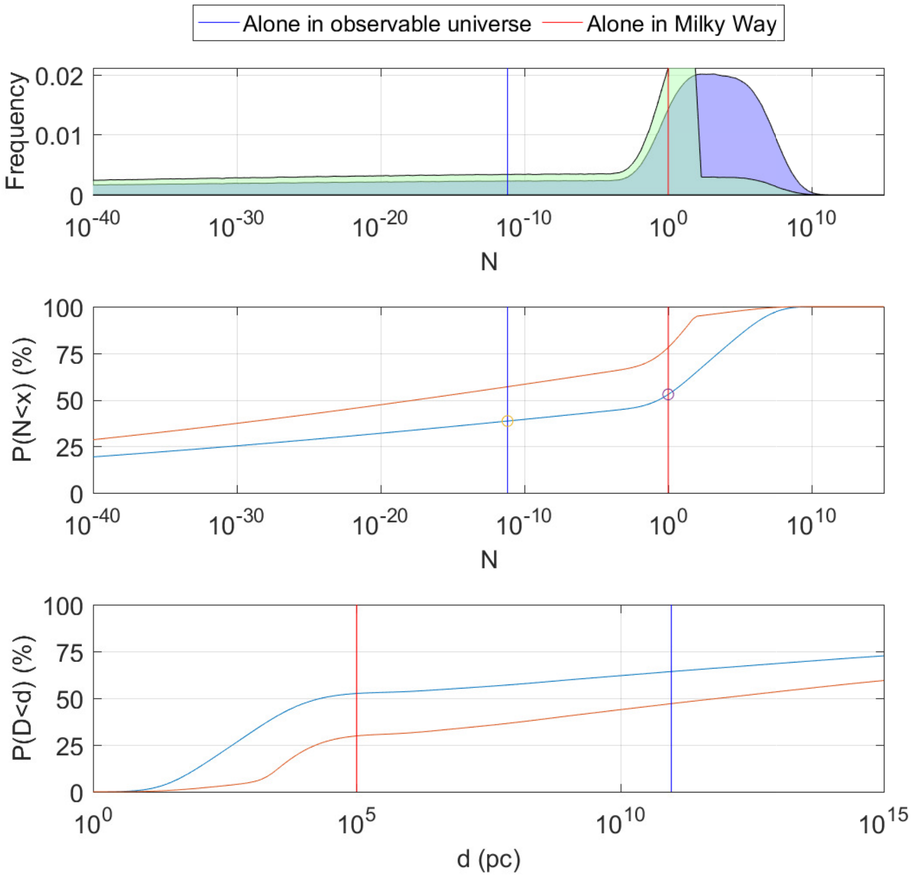


**Figure 6.** Effect of cut-off model of the Fermi observation, $N_0 = 100, p_{fail} = 0.1$.

region:

$$\Pr[\neg D|N, L < T] \approx e^{-N} + (1 - e^{-N}) \left(1 - \frac{L^\alpha}{(\alpha+1)T^\alpha}\right)$$

for $L < T$ and

$$\Pr[\neg D|N, L > T] \approx e^{-N} + (T/L)(1 - e^{-N}) \left(\frac{\alpha}{\alpha+1}\right)$$

for $L > T$, where $2 < \alpha < 3$ is a geometric factor due to the shape of the galaxy. This update disregards the cases where there are two or more simultaneously expanding civilizations, and hence gives an overestimate of $\Pr[\neg D|N]$ for larger $N$; extra (speculative) assumptions on the effect of interacting ETI are needed to define a fully consistent model.

This model also has the conceptual drawback that it assumes a civilization can go extinct during expansion over interstellar scales, something that appears implausible. One way of handling this is to change the lower limit of the distribution of $L$ so $L \geq T$ (producing a more optimistic $N$ but subject to a stronger update), "slow long-lived expansion".

The strongest expansion model ("permanent settlement") assumes that once a civilization begins expanding in the galaxy it will never go extinct and will remain extant nearly everywhere (despite possibly local extinctions). This is not a Drake-equation compatible steady state model,

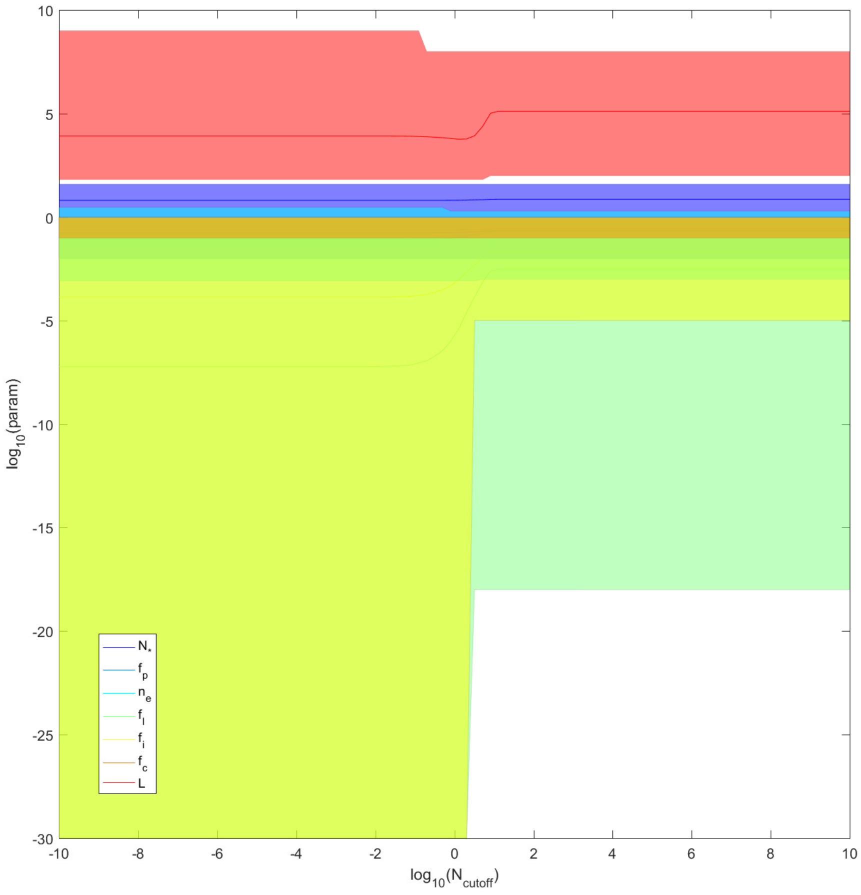


**Figure 7.** Effect on posteriors for the Drake equation parameters for a simple cut-off observation forcing $N < N_{cutoff}$. Filled regions correspond to 90% confidence intervals. Note how $f_l$ (yellow) is far more sensitive than $L$ (red), which in turn reacts more than the other parameters.

but can still be forced into the framework by assuming that our observations are only compatible with either that no other civilization has emerged during the history of the Milky Way, or that one has emerged less than time $T$ ago. Given an effective age $T_{MW}$ of the Milky Way (which can be adjusted to account for changing life-friendliness), the update becomes

$$\Pr[\neg D|N] \approx e^{-R^* f_p e_e f_l f_i f_c T_{MW}} = e^{-(N/L)T_{MW}}$$

if we ignore the recent emergence case[2]. Note that this update may *still* be too mild in the light of possible intergalactic colonization over long distances.

See figure 8 for a comparision of the different settlement updates. Overall, the effect is a very strong update towards extremely rare ETI, especially for the permanent settlement models.

[2]Since $T/T_{MW} < 0.003$ this is not a major correction. The full update ("permanent settlement or ongoing expansion") would be $\Pr[\neg D|N] \approx e^{-(N/L)(T_{MW}-T)} + (1 - e^{-(N/L)(T_{MW}-T)})(\alpha/(\alpha+1))$.

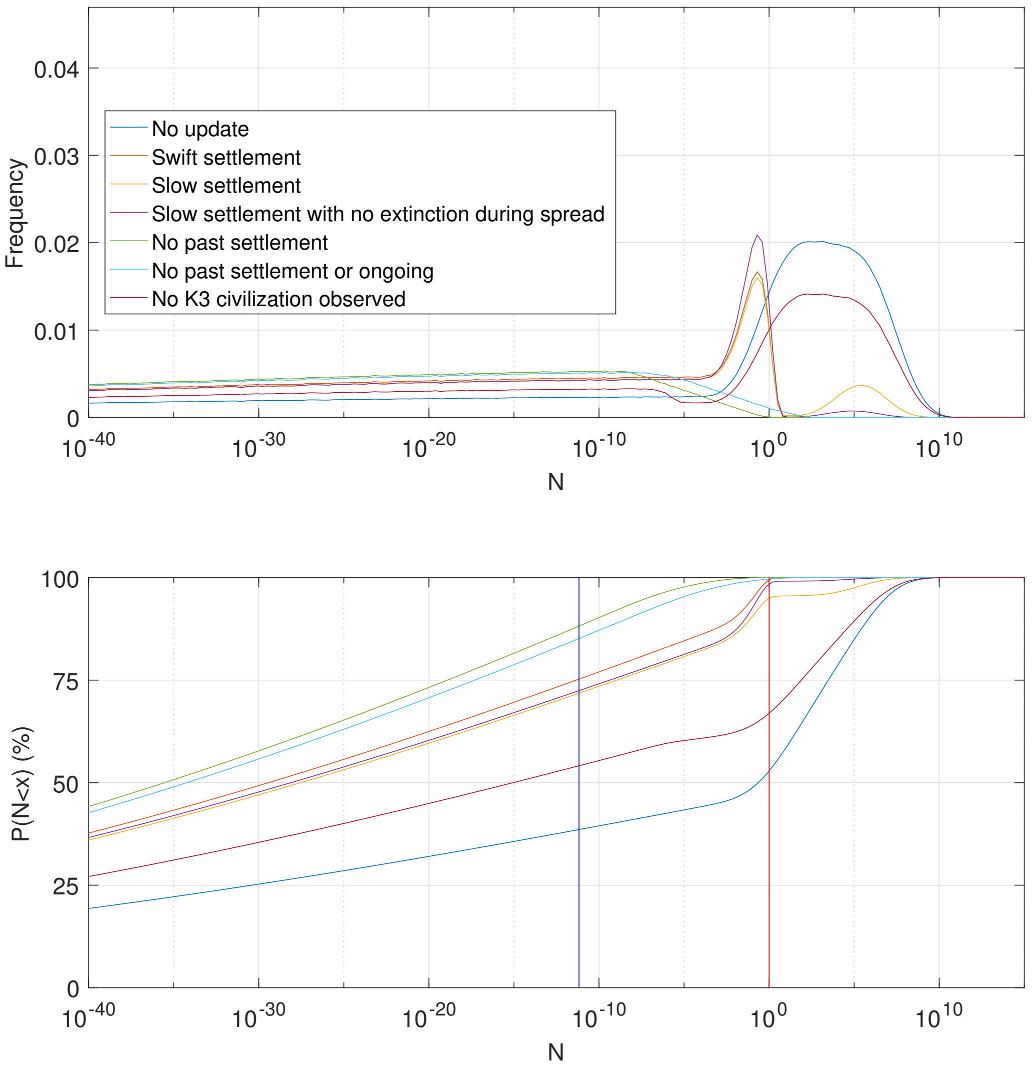


**Figure 8.** Effect of different settlement scenarios.

## Lack of observed K3 civilizations

A simple model of looking for advanced civilizations is that there exists a probability $p_1$ that it is desireable and feasible (for any species) to undertake massive galactic engineering, and a probability $p_2$ that any species that undertakes such a project will succeed[3]. Given $K$ observed galaxies with no sign of a K3 civilization, $\Pr[N|K] \propto [1 - p_1(1 - p_2^{KN})] \Pr[N]$.

The Ĝ-hat survey gives $K \approx 10^5$, effectively producing a cut-off of the credence in $N$ above $N \approx 10^{-5}$, with a strength dependent on $p_1$ and location mildly dependent on $p_2$. Setting $p_1 = 0.5$ to approximate a uniform prior produces a bimodal distribution of $N$, figure 9.

Using $p_1 = 0.5$ can also be seen as an approximation of a mixture distribution based on a $[0, 1]$ uniform prior of $p_1$.

[3]Models of fallible observations where there is probability $p_{detect}$ of noticing a civilization would replace $p_2$ with $p_2 p_{detect}$.

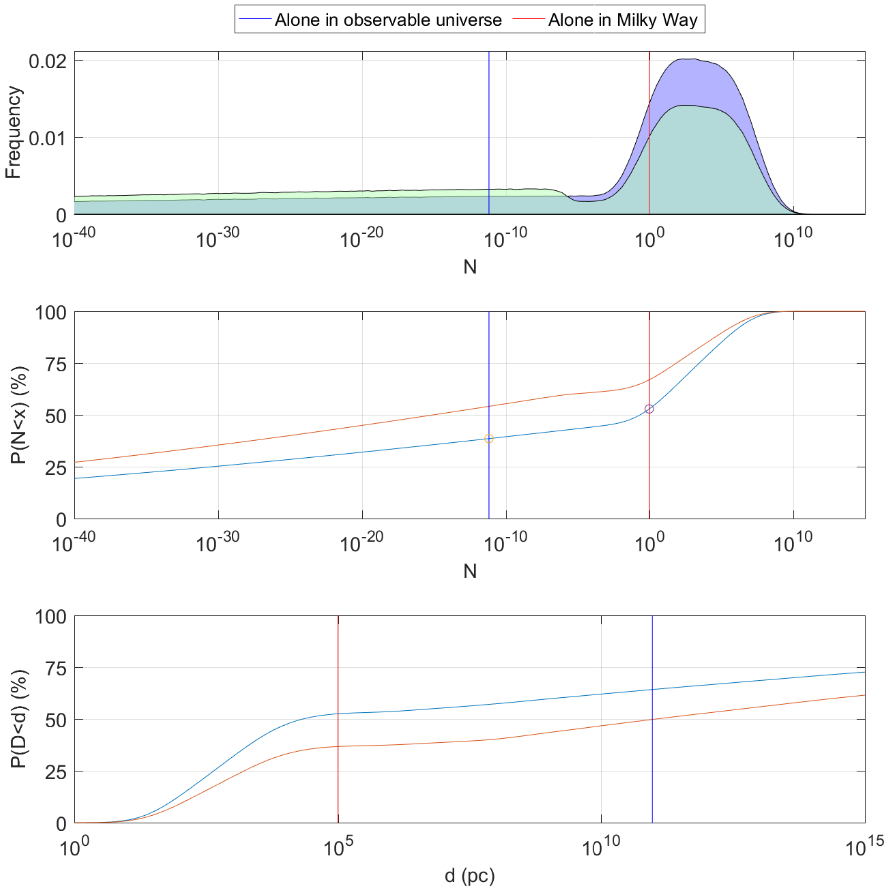


**Figure 9.** Effect of lack of observerd K3 civilizations in $10^5$ galaxies, assuming $p_1 = 0.5, p_2 = 0.01$.

## Positive observations

Discovering evidence would strongly affect the uncertainty distributions discussed in this paper. Clear evidence that bears on the parameters will reduce their uncertainty significantly, and hence update the distribution of N strongly.

### Dark biospheres

If an independently evolved âĂIJdark biosphereâĂİ was discovered on Earth (either alive or fossilized), this corresponds to the observation of at least one extra AGT over the lifespan of the biosphere. The posterior update of the rate of life emergence due to the observation is

$$\Pr[\lambda_l|\text{darkbiosphere}] \propto \Pr[dark|\lambda_l]\,\Pr[\lambda_l] = (1-e^{-\lambda_l})\,\Pr[\lambda_l].$$

Were $N$ independent forms of life found besides standard life the update is

$$Pr[\lambda_l|N\text{biospheres}] \propto \left(1 - e^{-\lambda_l}\sum_{n=1}^{N} \lambda_l^n/n!\right)\Pr[\lambda_l].$$

If just the $f_l$ fraction is used the update is instead $\Pr[f_l|N\text{biospheres}] \propto f_l^n \Pr[f_l]$.

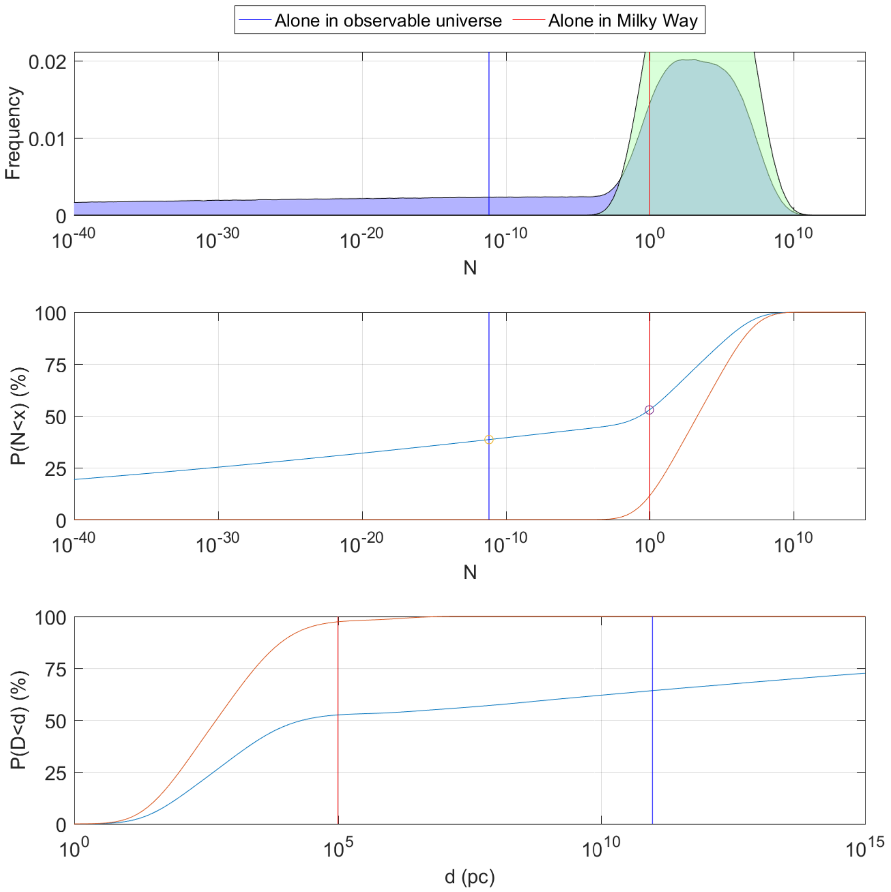


**Figure 10.** Effect of discovering one dark biosphere on Earth.

The main effect (figure 10) is to strongly cut off the low tail of $f_l$, while leaving $L$ invariant. This makes an early great filter less likely, although it may still be supplied by a very low value of $f_i$.

## Independent biosphere on Mars, Europa etc.

If an independently evolved biosphere is found on another planet in the solar system the effect on uncertainty is twofold. First, since with the exception of Mars, none of the other planets are regarded as terrestrial the range of $n_e$ increases, possibly by an order of magnitude. Second, this gives evidence that out of $K$ planets $k$ have life, producing a beta-distribution update:

$$\Pr[f_l|K,k] \propto f_l^k (1-f_l)^{K-k} \Pr[f_l].$$

Discovering an exoplanet with life would produce a similar update, but unless it was non-terrestrial, have no effect on $n_e$.

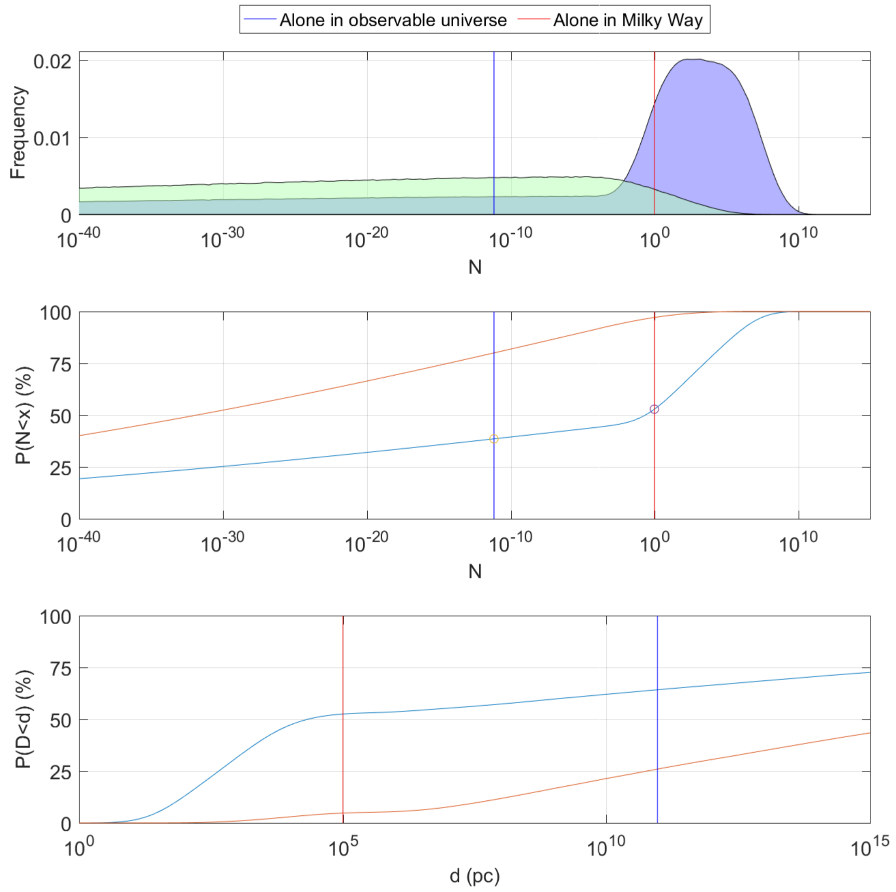


**Figure 11.** Effect of discovering one exoplanet biosphere out of 1000 sampled terrestrial planets.

The overall effect (figure 11) is to reduce the LU of $f_l$ by many orders of magnitude, with an effect on $N$ due to the fraction $k/K$ (and possible increases of $n_e$, causing a translation towards higher values by a factor $\approx 10$).

## No life on terrestrial planet

If we observe K Earth-like planets but find them empty of life, the update is simply

$$Pr[f_l|K] \propto (1-f_l)^K \operatorname{Pr}[f_l].$$

This corresponds to cutting off the âĂIJheadâĂİ of the $f_l$ distribution close to $f_l \approx 1$, while leaving $L$ unchanged, making an early great filter a very plausible explanation.

## Non-independent biosphere

Discovering a biosphere sharing genetic coding with Earth-life implies that interplanetary (if found in the solar system) or interstellar (if exoplanet) panspermia is possible or that there exist a strong convergence of coding systems. The first case implies at least a regional update of $f_l$ as above, but the full effect on $N$ depends on the characteristic size of panspermia

regions, something the observation itself does not fix. The second case reduces the likelihood of alternative, slowly evolving coding systems and hence increases $f_i$. Unfortunately this scenario is underconstrained, but would increase $f_l$ and $f_i$ by some factors.

## Prehistoric intelligence

Were we to find evidence for the existence (but not lifespan) of a pre-human indigenous intelligent species on Earth this would update $f_i$ as

$$\Pr[f_i|\text{artefacts}] \propto f_i \Pr[f_i],$$

a simple update of $f_i$. The overall effect is a translation of the $N$ distribution upwards, with no change in the relation between $f_l$ and $L$ (figure 12).

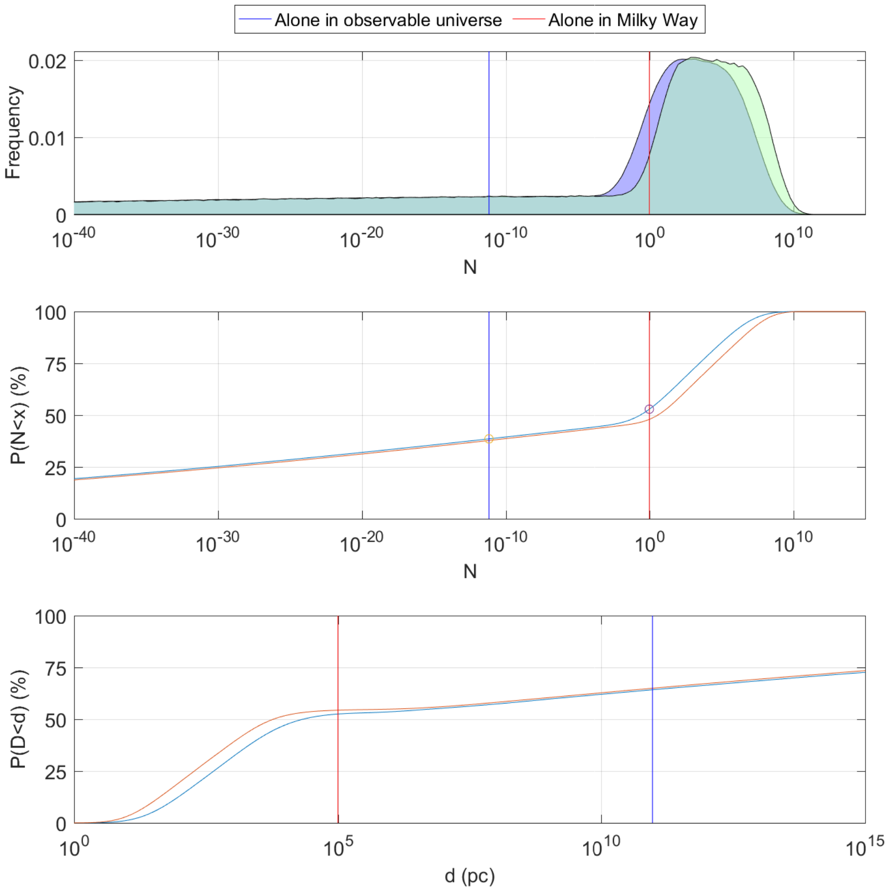


**Figure 12.** Effect of discovering one prehistoric civilization on Earth.

Note that more archaeological evidence would also have an effect on $L$ depending on the time $l$ the species was around; the minimum-variance unbiased estimate of a log-uniform L would be $\tilde{L} = 2l$.

## Alien ruins or artefacts

Finding signs of past intelligence on a non-Earth planet has a more complex effect. If the find was due to a species clearly local to the planet, the update is

$$\Pr[f_i|K, \text{ruins}] \propto f_i(1-f_i)^{K-1}\Pr[f_i]$$

(where $K$ other planets have been explored before).

However, if it is not clear from where the intelligence originated the update must be significantly weakened to take into account that it merely indicates at least one civilization emerging across the Milky Way (or past-accessible universe) at some point.

## Extant extraterrestrial intelligence in Milky Way

Discovery of an extant civilization in the Milky Way leads to the update cutting off N<2. The effect is a strong amplification of larger $N$, plus cutting of the low tail of $f_l$, with a weaker increase of $L$ (figure 13).

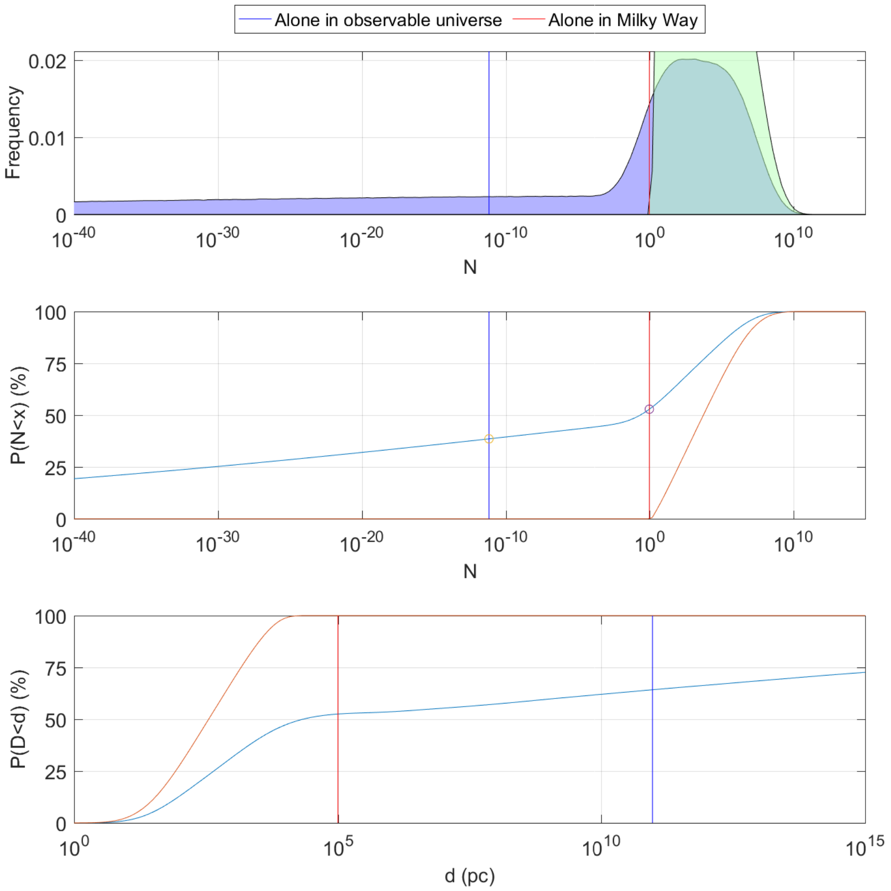


**Figure 13.** Effect of discovering one extant civilization in the Milky Way.

## Observation of intelligence outside Milky Way

This would correspond to a lower cut-off of $N$ at some point $N_{cutoff}$. One crude way of estimating $N_{cutoff}$ is to estimate it as 1/[the number of galaxies within the radius], or $N_{cutoff} = 3N_{MW}/4\pi\rho d^3$ where $\rho = 2.4 \times 10^{-8}\,\mathrm{pc}^{-3}$ is the average star density of the universe and $N_{MW} = 3 \times 10^{11}$ the number of stars in the milky way, implying $N_{cutoff} = 3 \times 10^{18}/d^3$.

For example, detecting galactic engineering at distance $100\,\mathrm{Mpc}$ implies $N_{cutoff} = 3 \times 10^{-6}$, while finding it in Andromeda ($778\,\mathrm{kpc}$) gives $N_{cutoff} = 6.3$ (which demonstrates that it overestimates civilization density at size scales corresponding to clusters). These cases have similar effects on parameters as the civilization in Milky Way case.

# Spatiotemporal correlations

As noted by Häggström and Verendel[4], if the prior factors in the Drake equation are strongly correlated, the effect of new evidence on the estimates changes and the strength of our belief in an early Great Filter may even decrease even if we find evidence for single-celled extraterrestrial life. This required somewhat extreme correlations, possibly representing a prior that the universe is either very welcoming of complexity on all levels (planets, life, intelligence, civilizations) or not.

Other ways of getting correlated priors are:

- A natural astrophysical correlation set by the assumption of life emerging near stars rather than in the warm intergalactic plasma or dark matter halos; this corresponds to a spatial correlation scale on the order of tens of kiloparsec (galaxies). Unless the other factors in the Drake equation produce typical distances between civilizations beyond the End of Greatness scale (hundreds of megaparsec), we should expect a spatially correlated structure of intelligent life following galaxies, clusters and filaments. However, this is already implicitly assumed by the Drake equation focus on the galaxy.
- Galactic habitable zones, if they exist, induce a correlation length on the order of 4-10 kpc.
- Panspermia naturally induces a spatial correlation scale $D_p$ making $f_l$ correlated (and higher) inside regions of spread. If the other factors produce typical distances between civilizations $d_c \approx 0.5(N/N_{MW})^{-1/3}$ larger than the typical panspermia diameter $D_p$ this spatial correlation is irrelevant. Conversely, if the distance within panspermias is much smaller than their diameter the local density has little spatial correlation (the Drake estimate of $N$ might be too optimistic if the panspermia is smaller than the galaxy, but the local density estimate will be correct). Panspermias hence affect correlations mainly if the typical civilization distance is within a relatively small range $d_c \approx D_p$. Since $D_p$ is determined solely by properties of panspermia dynamics and astrophysics, while $d_c$ is determined by independent factors of astrophysics and biosphere development, this coincidence is relatively unlikely.
  It is also relevant to note that the timescale of panspermia expansion in the Milky Way, assuming a spread speed on the order of interstellar dust ($26\,\mathrm{km\,s}^{-1}$), is about half a billion years. Given an age of the galaxy as $13.6\,\mathrm{Gyr}$ this gives less than a 1 in 27 chance of us living in an era of incomplete panspermia.
- Due to the accelerating expansion of the universe there exists an upper limit to how far any civilization traveling below lightspeed can reach and hence induce correlations[5]. This distance is dependent on time of origin (currently $<5\,\mathrm{Gpc}$), with early civilizations potentially able to cause correlations of significant cosmological distances.

[4]Verendel, V., & Häggström, O. (2016). Fermi's paradox, extraterrestrial life and the future of humanity: a Bayesian analysis. International Journal of Astrobiology, 1-5.
[5]Armstrong, S., & Sandberg, A. (2013). Eternity in six hours: Intergalactic spreading of intelligent life and sharpening the fermi paradox. Acta Astronautica, 89, 1-13.

- Temporal synchronization via GRBs/supernovas[6] make the appearance of advanced life correlated in time, possibly inducing a phase transition from a low $f_i$ to a higher $f_i$. This acts mostly to cut off the effect of very long lived civilizations, and weakens the intergalactic colonization update.
- If civilizations prevent each other from coming into being (a common assumption for interstellar settlement models, including our posterior update), then $N$ tends to be either 0 or 1 at any point in time in a colonizable region, unless an unlikely coincidence occurs during an expansion phase. This sets a temporal correlation length $\approx L$ and a spatial correlation length based on the size of the settlement.
- Spatiotemporal time and longevity correlations can also be induced by models such as Brin's resource exhaustion model[7] or percolation spread models[8]. Here the natural scale is set by how the colonization dynamics produce colonized (new civilizations precluded), uncolonized (no change in civilization formation rate) and depleted (lowered formation rate over a certain timespan) regions.

Any no-detection update with a characteristic detectability horizon in space or time will be insensitive to correlations with smaller correlation distances or times. It also does not directly indicate anything about the possibility of very different parameters outside its limits.

## Observer selection effects

However, there is an observer selection effect favoring observers finding themselves in the richer regions of spacetime. If the density of civilizations is $\rho_1$ in a volume fraction $V$ and $\rho_2$ elsewhere, the probability that an observer is in a type-1 region is $\Pr[1] = \rho_1 V/(\rho_1 V + \rho_2(1-V))$ and the ratio is $\Pr[1]/\Pr[2] = (\rho_1/\rho_2)(V/(1-V))$. The mean *observed* density will be $\hat{\rho} = (\rho_1^2 V + \rho_2^2(1-V))/(\rho_1 V + \rho_2(1-V))$ while the actual mean density will be $\bar{\rho} = \rho_1 V + \rho_2(1-V)$. Hence the relative overestimation of $\bar{\rho}$ for region-1 observers will be

$$\hat{\rho}/\bar{\rho} - 1 = \frac{(\rho_1/\rho_2)^2 V + 1 - V}{((\rho_1/\rho_2)V + 1 - V)^2}.$$

This increases linearly in $\rho_1/\rho_2$ and has a maximum for $V = 1/((\rho_1/\rho_2)+1)$ (Figure 14).

Unless the ratio $\rho_1/\rho_2$ is $\gg 1$ the error factor is not going to dominate the probability updates. Were the ratio very high, however, the volume range where this occurs would be small. It is hence *a priori* unlikely to get very erroneous estimates due to the observer selection effect unless there is some other correlation forcing the right density-volume relationship.

[6]Annis, J. 1999a, âĂİAn Astrophysical Explanation for the Great Silence,âĂİ J. Brit. Interplan. Soc. 52, 19-22 (preprint astro-ph/9901322).; Ćirković, M. M., & Vukotić, B. (2008). Astrobiological phase transition: towards resolution of FermiâĂŹs paradox. Origins of Life and Evolution of Biospheres, 38(6), 535-547.
[7]Brin, G. D. (1983). The great silence-The controversy concerning extraterrestrial intelligent life. Quarterly Journal of the Royal Astronomical Society, 24, 283-309.
[8]G.A. Landis (1998) The Fermi paradox: an approach based on percolation theory. J Br Interplanet Soc 51:163âĂŞ166.

rspa.royalsocietypublishing.org Proc R Soc A 0000000

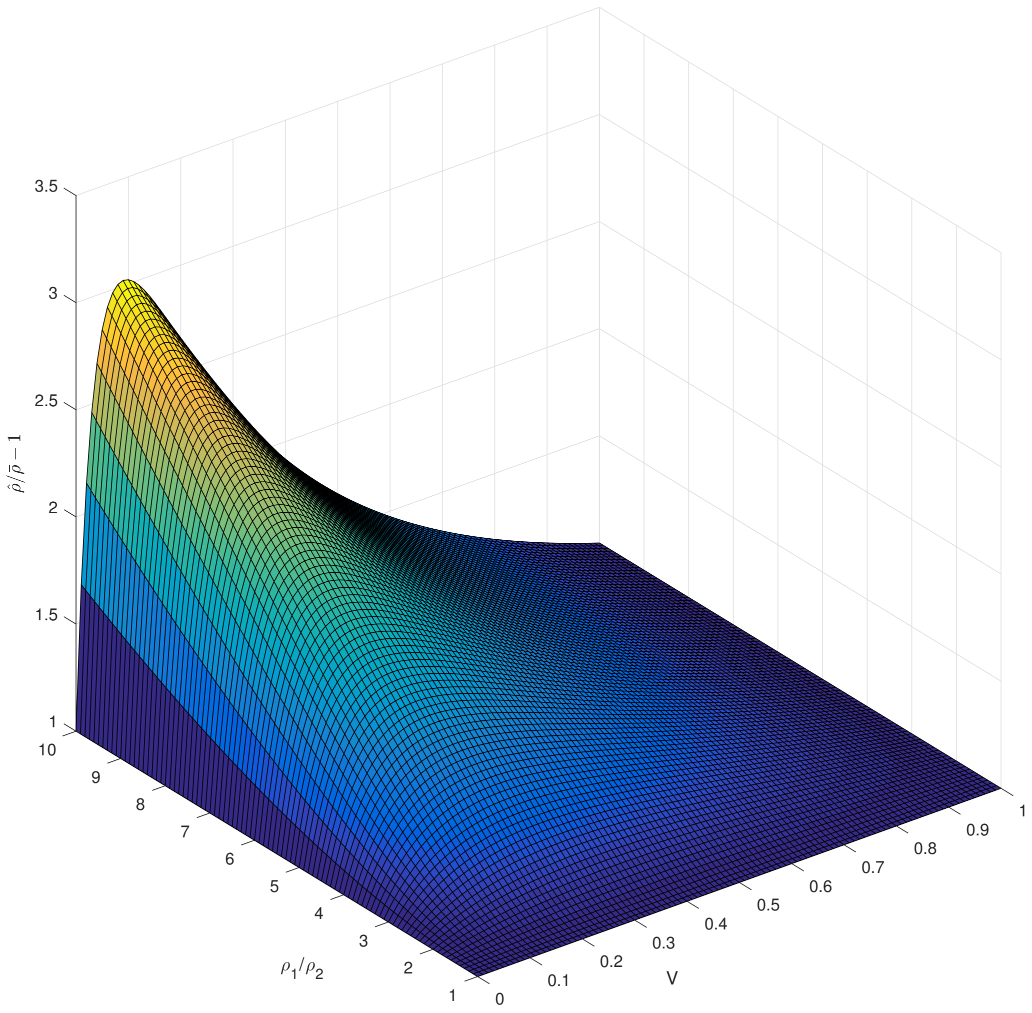


**Figure 14.** Observer selection effects inducing overestimates of civilization density as a function of volume fraction in enriched regions ($V$) and density ratio ($\rho_1/\rho_2$).
