# Supplementary material for: Dissolving the Fermi Paradox
Source: arXiv:1806.02404 ancillary file (2018-06-06)
Supplement: Supplementary file 3 [file supplement-iii-drake.pdf]

PROCEEDINGS A

rspa.royalsocietypublishing.org

Research

Article submitted to journal

# Supplement III: Drake equation parameter estimates in the literature

Anders Sandberg[1], Eric Drexler[1] and Toby Ord[1]

[1]Future of Humanity Institute

THE ROYAL SOCIETY
PUBLISHING

© The Authors. Published by the Royal Society under the terms of the Creative Commons Attribution License http://creativecommons.org/licenses/by/4.0/, which permits unrestricted use, provided the original author and source are credited.

## Data sources

The literature review consisted of searching through the scientific literature using Google Scholar for mentions of the âĂIJDrake equationâĂİ and âĂIJparametersâĂİ. Books and papers found via these sources were also considered.

## Data handling

Alternative forms of the Drake equation have insofar possible been converted to the standard form. In some cases terms have been merged (such as products expressing $n_e$ as a result of several factors).

The exact meaning of $f_p$ and $n_e$ varies between authors; we have not attempted to refine these meanings.

Star formation rates given as solar masses have been converted to stars by assuming an average stellar mass of 0.7 solar masses.

The papers giving ranges have been entered as two estimates (high and low) for each parameter.

## Data quality

It should be noted that the estimates are not independent, since many authors base their estimates on updates of previously published estimates. This introduces an artificial variance reduction to the collective estimate.

There is also a clear bias present towards optimistic, high values since SETI or ETI skeptics typically do not give estimates.

## Data properties

The range of values are $R^*$: [1,50], $f_p$: [$10^{-2}$,1], $n_e$: [$2.8 \times 10^{-6}$,10], $f_l$: [$10^{-30}$,1], $f_i$: [$10^{-30}$,1], $f_c$: [$10^{-2}$,1], $L$: [45,109].

The medians are $R$:10, $f_p$: 0.333, $n_e$: 0.5, $f_l$: 0.5, $f_i$: 25, $f_c$: 0.25, $L$: $10^5$.

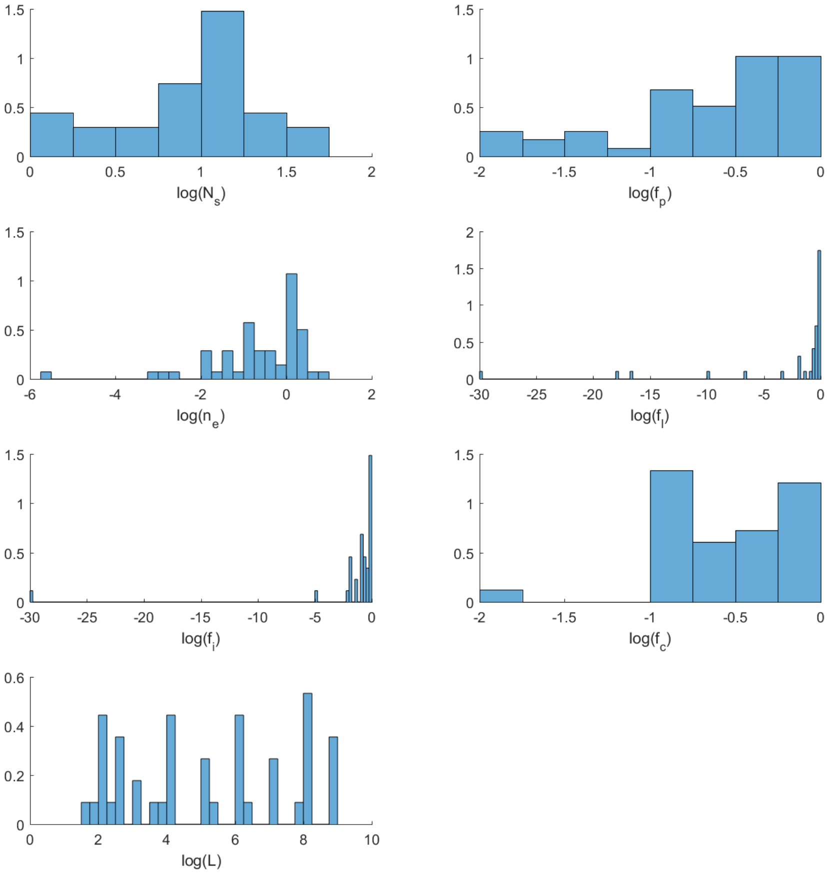


**Figure 1.** Histogram plots of the distribution of Drake equation parameter values found in the literature. Beside a few outliers, note the narrow ($\approx 2$ orders of magnitude) distribution of the highly uncertain life, intelligence and communications factors.

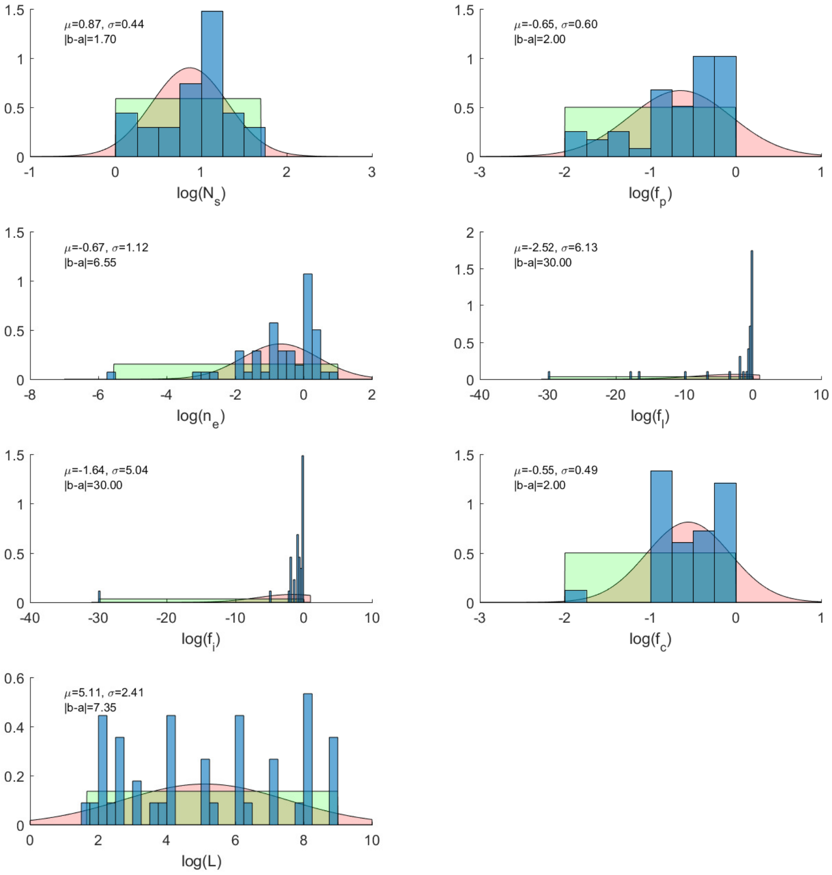


**Figure 2.** Fits of uniform and normal distributions to estimates in literature.
