# Supplementary material for: Dissolving the Fermi Paradox
Source: arXiv:1806.02404 ancillary file (2018-06-06)
Supplement: Supplementary file 4 [file supplement-iv-conditioning.pdf]

PROCEEDINGS A

rspa.royalsocietypublishing.org

Research

Article submitted to journal

# Supplement IV: Conditioning on a non-large joint tail moves the most uncertain component the most

Anders Sandberg[1], Eric Drexler[1] and Toby Ord[1]

[1]Future of Humanity Institute

© The Authors. Published by the Royal Society under the terms of the Creative Commons Attribution License http://creativecommons.org/licenses/by/4.0/, which permits unrestricted use, provided the original author and source are credited.

THE ROYAL SOCIETY
PUBLISHING

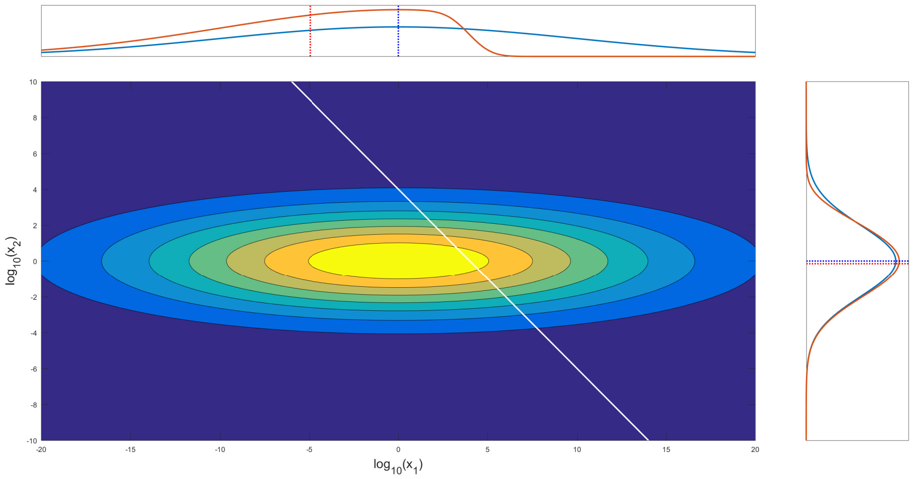


**Figure 1.** A simple model, where two parameters (e.g. rate of life formation and number of Earth-like planets) have Gaussian credence distributions in log-space, producing the joint distribution at the centre and the marginal distributions (blue) at the sides. If we condition on their product being smaller than a certain value (white line), conditional marginal distributions (red) are produced. The means differ far more for the broadly distributed variable than for the narrowly distributed variable.

Let $X_i$ be independent random variables with density functions $f_i(x_i)$, forming a joint multivariate distribution $f(x_1, x_2, \ldots, x_n) = \prod_{i=1}^n f_i(x_i)$. Given that the sum[1] of the variables is less than some threshold, we are interested in how much the posterior distributions $f_i(x_i | \sum_{j=1}^n x_j < \theta)$ shift relative to the priors.

Letting $y = \sum_{j=2}^n x_j$ and $x = x_1$ this can be treated as the 2D case

$$f_x(x|x+y<\theta) = \frac{\int_{-\infty}^{\theta-x} f(x,y)dy}{\int_{-\infty}^{\infty}\int_{-\infty}^{\theta-x} f(x,y)dydx} = \frac{A(\theta)}{B(\theta)},$$

where the first integral is

$$A(\theta) = f_x(x)\int_{-\infty}^{\theta-x} f_y(y)dy = f_x(x)F_y(\theta-x).$$

The normalisation integral $B(\theta)$ is

$$B(\theta) = \int_{-\infty}^{\infty}\int_{-\infty}^{\theta-x} f(x,y)dydx = \int_{-\infty}^{\infty} f_x(x)F_y(\theta-x)dx =$$
$$= (f_x * F_y)(\theta).$$

Conversely, $f_y(y|x+y<\theta) = f_y(y)F_x(\theta-y)/(f_x * F_y)(\theta)$.

Narrow distributions experience conditioning as rescaling (largely removed by normalization), while broad distributions experience it as cutting off the upper tail.

The change in expectation (if it exists) is

$$\Delta E(\theta) = E[x] - E[x|\theta] = \int_{-\infty}^{\infty} x f_x(x)\left[1 - \frac{F_y(\theta-x)}{(f_x * F_y)(\theta)}\right]dx.$$

[1]Conditioning on bounds on the sum of the variables in log-space corresponds to conditioning on bounds of their products in normal space.

For $E[x] = 0$ this simplifies to

$$\Delta E(\theta) = -\frac{(xf_x * F_y)(\theta)}{(f_x * F_y)(\theta)}.$$

It should be noted that this does not apply to all distributions: multimodal distributions or ones lacking expectation (such as the Cauchy distribution) do not respond to conditioning in the monotonic manner discussed here. However, it is applicable to the two key cases of Gaussian and uniform random variables.

## Gaussian distributions

In the case where $x$ and $y$ are Gaussian, if we set $\mu_x = \mu_y = 0$ and use $t = x/\sigma_x^2$, $\Delta E(\theta)$ can be evaluated in explicit form[2]:

$$(f_x * F_y)(\theta) = \frac{1}{\sigma_x^2}\int_{-\infty}^{\infty} \phi(t)\Phi\left(\frac{\theta - \sigma_x^2 t}{\sigma_y^2}\right) dt =$$

$$\frac{1}{\sigma_x^2}\Phi\left(\frac{\theta}{\sqrt{\sigma_y^2 + \sigma_x^4/\sigma_y^2}}\right)$$

$$(xf_x * F_y)(\theta) = \int_{-\infty}^{\infty} t\phi(t)\Phi\left(\frac{\theta - \sigma_x^2 t}{\sigma_y^2}\right) dt =$$

$$-\frac{\sigma_x^2}{\sqrt{\sigma_y^2 + \sigma_x^4/\sigma_y^2}}\Phi\left(\frac{\theta}{\sqrt{a_y^2 + \sigma_x^4/\sigma_y^2}}\right)$$

where $\phi(x) = (1/\sqrt{2\pi})e^{-x^2/2}$ and $\Phi(x) = \int_{-\infty}^{x} \phi(t)dt = (1/2)(1 + \mathrm{erf}(x/\sqrt{2}))$.

Hence:

$$\Delta E(\theta) = -\frac{\sigma_x^4}{V}\frac{\phi(\theta/V)}{\Phi(\theta/V)}$$

where $V = \sqrt{\sigma_y^2 + \sigma_x^4/\sigma_y^2}$. $\Delta E(\theta)$ approaches zero for large positive theta, while the behavior on the negative side is asymptotically linear. Note that the magnitude of the shift in expectation quadratically depends on $\sigma_x^2$: if it is larger than $\sigma_y^2$ the change in expectation will be larger (figure 2).

## Distributions supported on a bounded interval

For a (well behaved) probability distribution with $f(x) > 0$ for $a \le x \le b$ the average expectation change $\Delta E/\Delta\theta$ when $\theta$ changes from $b$ to $a$ is bounded by $(E[x] - a)/(b - a)$. Hence if $x$ has a broader support than $y$, the expectation change in $x$ will typically be larger than for $y$ on average.

## Uniform distributions

Uniform distributions can be seen as bounds on distributions with finite support. With no loss of generality, consider the 2D case of two uniform distributions with mean 0 and range $x \in [-a, a]$, $y \in [-b, b]$. Depending on the value of $\theta$ there are five cases:

### Case 1

For $\theta > a + b$ the distributions are unchanged: $E[x|\theta] = 0$, $E[y|\theta] = 0$, $\Delta E(\theta) = 0$.

[2]Owen, D. B. (1980). A table of normal integrals: A table. Communications in Statistics-Simulation and Computation, 9(4), 389-419.

rspa.royalsocietypublishing.org Proc R Soc A 0000000

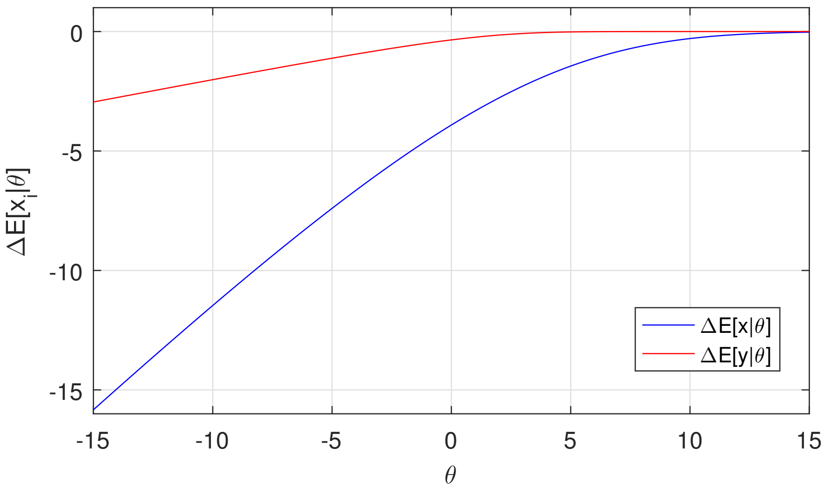


**Figure 2.** Response of joint Gaussian distribution to conditioning $x+y<\theta$, where $x \sim N(0,5)$ and $y \sim N(0,1)$.

## Case 2

For $a+b>\theta>a-b$ the condition cuts off a triangular corner of the joint distribution from $(\theta-b, b)$ to $(a, \theta-a)$. Projecting on the x-axis and normalizing gives

$$E[x|\theta] = \frac{-(2a-b+\theta)(a+b-\theta)^2}{3(-a^2+6ab+2a\theta-b^2+2b\theta-\theta^2)}$$

and conversely for $y$:

$$E[y|\theta] = \frac{-(2b-a+\theta)(a+b-\theta)^2}{3(-a^2+6ab+2a\theta-b^2+2b\theta-\theta^2)}$$

## Case 3

For $a-b>\theta>-a+b$ the condition leaves a right trapezoid with base $\theta+a+b$, top $\theta+a-b$, and altitude $2b$. Projecting on the x-axis and normalizing gives

$$E[x|\theta] = -a + \frac{3a^2+6a\theta+b^2+3\theta^2}{6(\theta+a)}.$$

Projecting on the y-axis and normalizing gives a right trapezoid:

$$E[y|\theta] = \frac{-b^2}{3(\theta+a)}.$$

## Case 4

For $-a+b>\theta>-(a+b)$ the condition cuts off everything but the lower triangular corner of the joint distribution, producing

$$E[x|\theta] = -a + (a+b+\theta)/3$$

$$E[y|\theta] = -b + (a+b+\theta)/3$$

## Case 5

For $\theta < -(a+b)$ the condition is inconsistent.

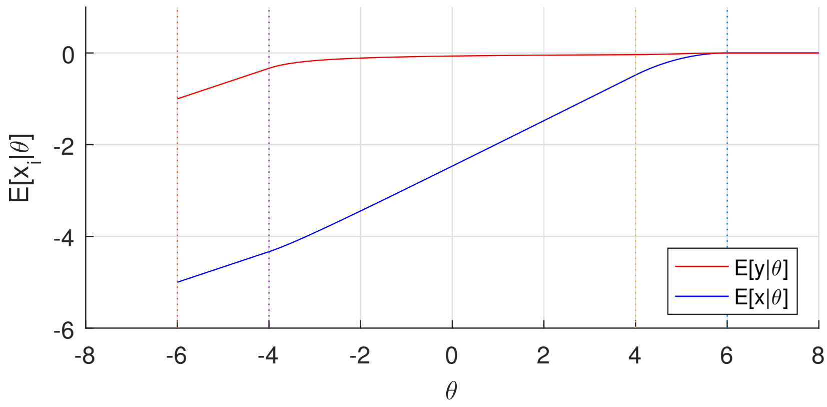


**Figure 3.** Response of joint uniform distribution to conditioning $x+y<\theta$, where $x\sim U(-5,5)$ and $y\sim U(-1,1)$. Vertical dotted lines denote the borders between different intersection cases.

## Effect on relative response

For case 3 (covering the largest interval of $\theta$)

$$E'[x|\theta]=1-\frac{3a^2+6a\theta+b^2+3\theta^2}{6(a+\theta)^2}\approx 1/2$$

and

$$E'[y|\theta]=\frac{b^2}{3(a+\theta)^2}\approx 0,$$

where the approximations apply for $a\gg b$. In this range $E'[x|\theta]>E'[y|\theta]$ if $a>b$, making the x-response significantly larger than the y-response (figure 3).
